# Supplementary material for: Fiduciary Duty in the Municipal Bonds Market
Source: arXiv:2406.15197 source file (2024-06-21)
Supplement: Supplementary file 1 [file Appendix.tex]

\setcounter{table}{0}
\setcounter{page}{0}

\setcounter{figure}{0}

\setcounter{section}{0}
\setcounter{equation}{0}

\clearpage
% \linespread{0.8}
\doublespacing
		
\section{Advisor Names}\label{sec:adv_names}
There is substantial variation in the names used by FTSE Russell to record municipal advisors. Often these variations are due to spellings like ``BACKSTORM MCCARLEY BERRY \& COMPANY LLC'' vs ``BACKSTROM MCCARLEY BERRY \& COMPANY''. We investigate the bond offer statement associated with the CUSIP to verify the corresponding entity and update the standardized name. Besides the jumbled spelling errors, we also come across typos and mistakes due to omitted letters. For example, ``BERKSHIRE BANK'' and ``BERSHIRE BANK'' correspond to the same municipal advisor. Further, we also account for alternative company name extensions, such as, ``LLC'', ``INC'', ``Co.'' or ``CO.''. These extensions are recorded differently over time for the same company. Occasionally, the names would omit portions of the names altogether: ``SUDSINA \& ASSOCIATES'' was also reported as ``SUDSINA''. To verify against mismatching firm names, we rely on logos printed on the bond's offering statement in addition to the official address provided. 
% The address typically includes the name of the city and state.

Other instances of spelling differences involve special characters like ``.'' or ``,'' and ``\&''. Clearly, these are easy to handle and to resolve. We also need to update names for subsidiaries and affiliated company names. These would also often involve mergers and acquisitions. Following \cite{cestau2020specialization}, we retroactively replace the names of the merged entities with the name of the new company. To an extent, this assumes that client relationships prevailed even after the M\&A activity. Indeed we do find evidence where both sets of names are found in the offering statements. This could also be due to delay in sale of bonds, especially via negotiation. Thus, offer statements may reflect contractual engagements before or after the merger activity. As a result, we identify these entities under a common name: for example, ``MERRILL LYNCH \& COMPANY'' and ``BANC OF AMERICA SECURITIES'' as ``BANC OF AMERICA SECURITIES''. We also find limited anecdotal evidence suggesting that acquisitions involve retention of officials in the new company.

Still other challenges include names where firms operate using different brand names. For example, ``SUSAN D. MUSSELMAN INC'', ``SDM ADVISORS INC'' and ``DASHENMUSSELMAN INC'' are captured differently. However, we represent them as ``A DASHEN \& ASSOCIATES'' by checking the names of principals and office locations recorded under each company. We believe that it is very difficult to identify abbreviated names corresponding to the same umbrella company without verifying each name separately. In some cases, we need to ascertain the office locations from internet search versus that reported in the bond offering statement. But we also come across simpler associations where alternative trading names used by companies are seemingly related, such as, ``RV NORENE \& ASSOCIATE INC'' and ``CROWE NORENE''. 

\clearpage
\linespread{0.4}
	\newpage {\footnotesize
		\putbib
		}

\clearpage
    \newpage
\begin{figure}
\begin{center}
\textbf{Total Issuance: Negotiated vs Competitive}
\end{center}
\centering
\includegraphics[scale=0.85]{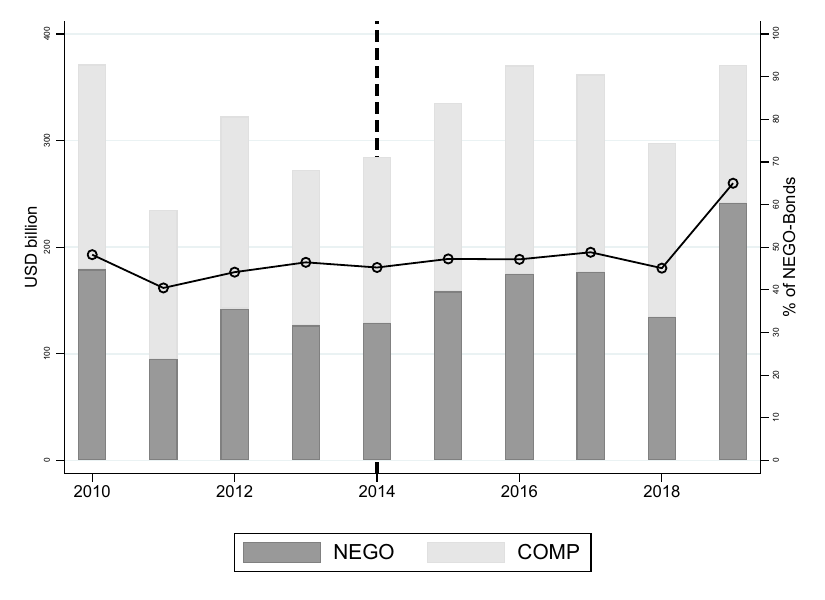}

\caption{\footnotesize{This figure shows the annual amount of advised bonds sold via negotiation. The left hand axis corresponds to the vertical bars denoting the amounts in USD billion. The line graph represents the percentage of dollar value sold via negotiation, shown on the right axis.}}
\label{fig:amt_nego}
\end{figure}

\begin{figure}
\begin{center}
\textbf{Likelihood of Negotiated Sale}
\end{center}
\centering
\includegraphics[scale=0.85]{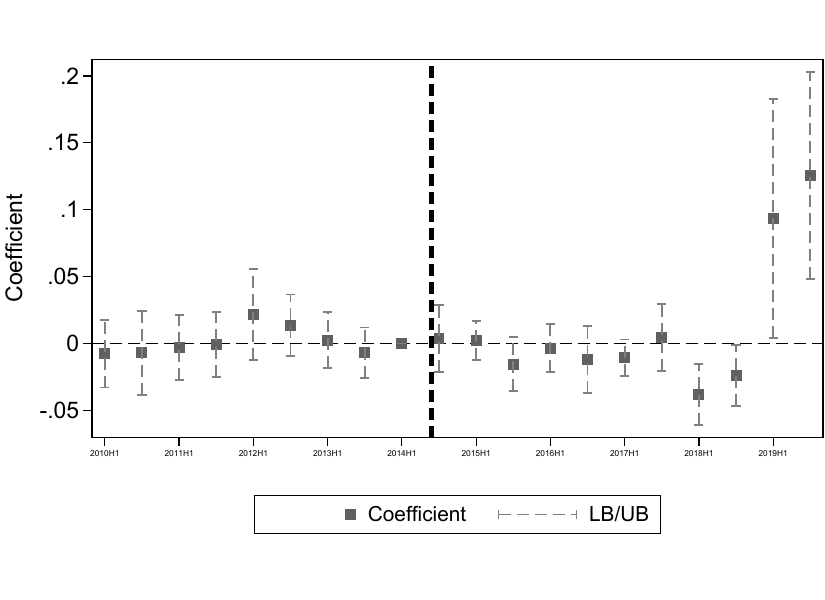}

\caption{\footnotesize{This figure reports the likelihood of issuing a bond via negotiation, \textit{within} issuer. We use the half-year period before the SEC Municipal Advisor Rule as the benchmark period. Standard errors are clustered at the state level.}}
\label{fig:ll_nego}
\end{figure}

\begin{figure}
\begin{center}
\textbf{Raw Binscatter of Offering Yields}
\end{center}
\centering
\includegraphics[scale=1.2]{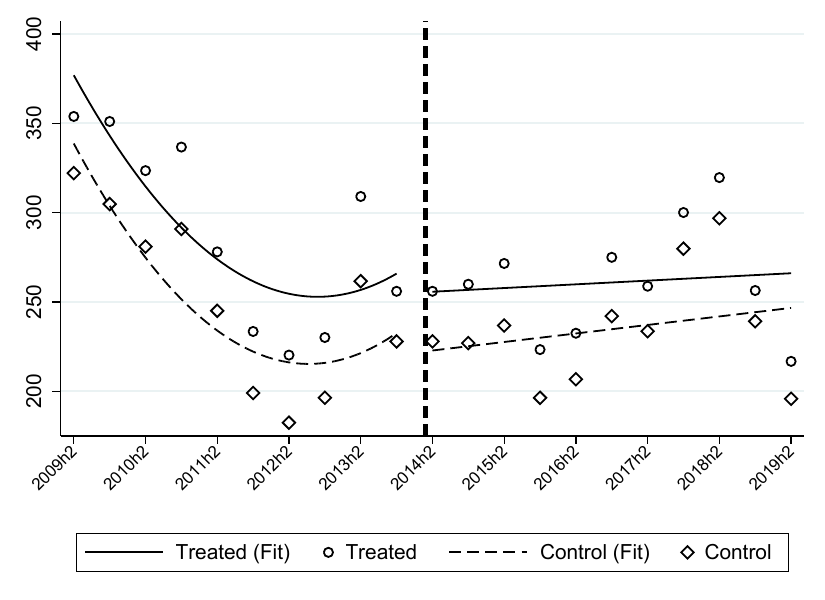}
% \label{fig:muni_adv_fees}

\caption{\footnotesize{This figure reports the binscatter of offering yields  in basis points on the y-axis. Each dot is the average of the offering yields calculated on every $5^{th}$ percentile of the sample for treated and control bonds, separately. The observed pattern suggests a convergence of yields between the treated and control bonds after the SEC Municipal Advisory Rule. This analysis should be interpreted in a non-causal way, as no fixed effect and controls are included.}}
\label{fig:bin_yields}
\end{figure}

\begin{figure}
    \raggedright\textbf{Offering Yields}\\
    \begin{subfigure}{\linewidth}
    \centering
    \includegraphics[scale=.7]{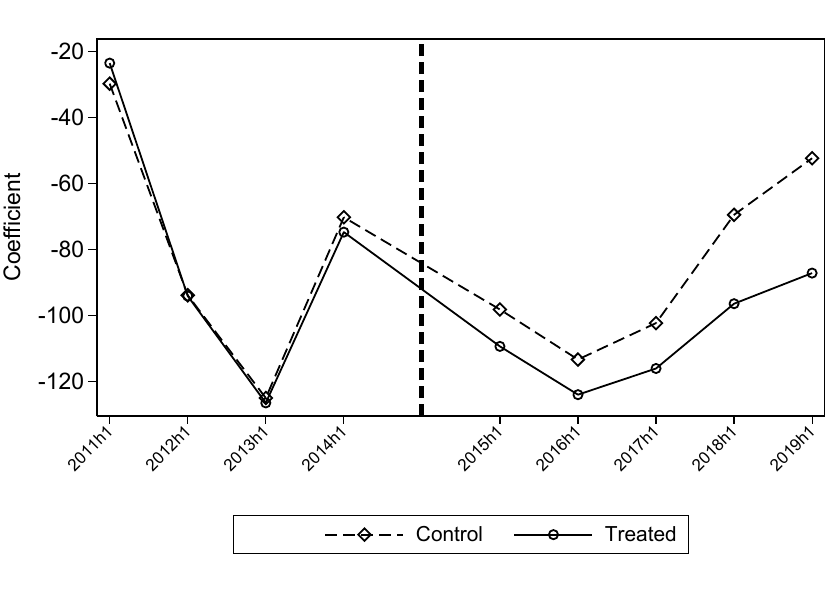}
    
    \caption{} 
    % \label{fig:issuance}
    \end{subfigure}
    
    \medskip
    \raggedright\textbf{Difference in Offering Yields}\\
    \begin{subfigure}{\linewidth}
    \centering
    \includegraphics[scale=.7]{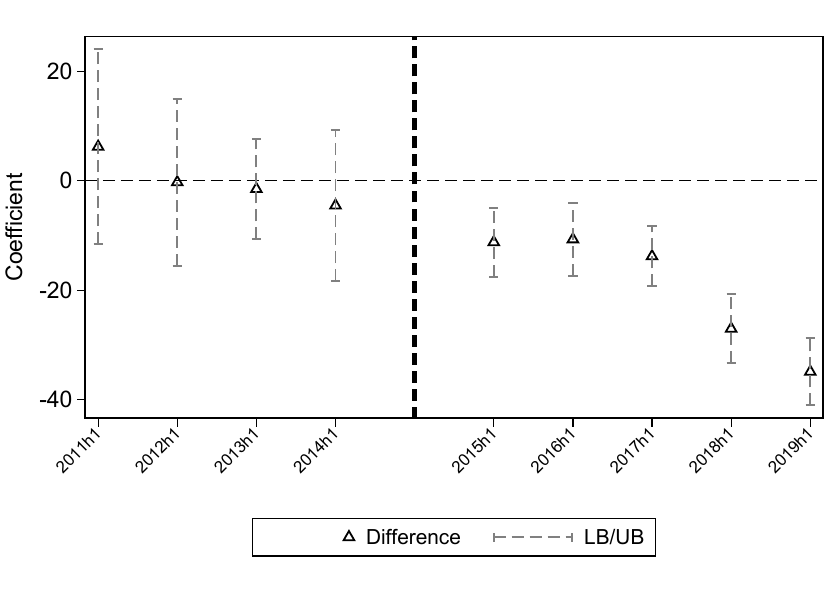}
    \caption{} 
    % \label{fig:issuance_byDebt}
    \end{subfigure}
    
\caption{\textbf{Baseline Result - Treated vs Control}: \footnotesize{In this figure, we plot the average offering yield for new municipal bonds using Equation \eqref{eq:dyn_yield_CompNego} in Panel (a). We also show the differences between the yields of treated and control bonds in Panel (b). See Table \ref{table:vardescription} for variables description. The coefficients are shown in basis points. Specifically, we regress the average yields on yearly interaction dummies for treated and control bonds using issuer-adviser pair fixed effects. We depict these coefficients on a yearly scale on the x-axis, where the vertical line corresponds to the Municipal Advisor Rule. The omitted benchmark period is the twelve month period before the event window shown above. Standard errors are clustered by state. The dashed lines represent 95\% confidence intervals.}}
\label{fig:did_yield}
\end{figure}

\begin{figure}
\begin{center}
\textbf{Refunding vs Refunded bonds}
\end{center}
\centering
\includegraphics[scale=1.2]{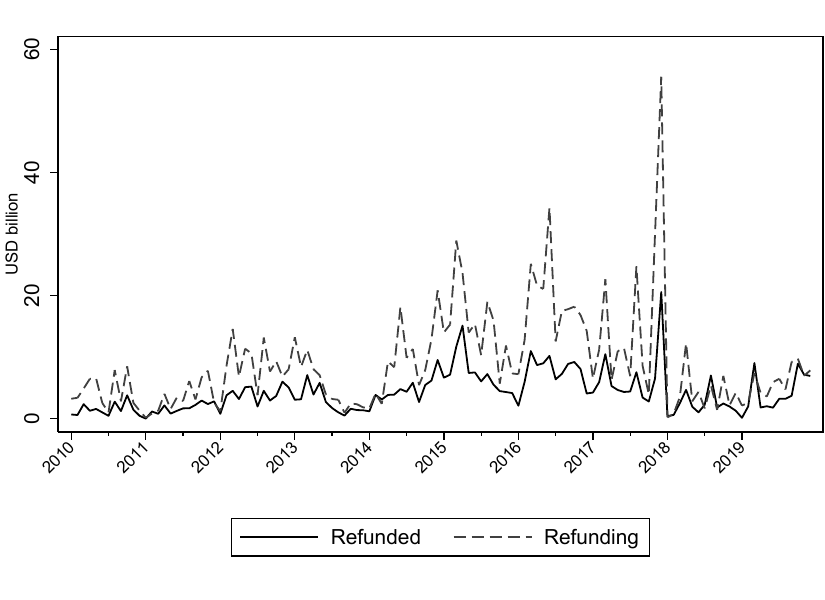}
% \label{fig:muni_adv_fees}

\caption{\footnotesize{This figure plots the monthly time series of the total par amount of municipal bonds refunded, as well as the refunding volume. Par amounts are
expressed in billions of dollars.}}
\label{fig:par_refund}
\end{figure}

\clearpage

\newpage
\clearpage

\begin{table}[htbp]
\def\sym#1{\ifmmode^{#1}\else\(^{#1}\)\fi}
\caption{Probability of Choosing Negotiated Sale Conditional on Ex-ante Observables}
%See table: Table10__calling_typeL_CCtrl_diff_refIssue_w1
\label{table:like_nego}
\vspace{0.2in}
\par
{\footnotesize This table shows the estimates from a linear probability regression of choice of negotiated sale on issue characteristics. See Section \ref{subsec:selecting_nego} for details. T-statistics are reported in brackets and standard errors are clustered at the state level. \sym{*} \(p<0.10\), \sym{**} \(p<0.05\), \sym{***} \(p<0.01\)}\\
% \vspace{.2in}
\vspace{.05in} 
% \resizebox{0.9\textwidth}{!} {

% \raggedright\textbf{Panel A: Primary Market}\\
\vspace{0.1in}
\centering
\resizebox{0.7\textwidth}{!} {
\begin{tabular}{@{\extracolsep{4pt}}l*{6}{c}}
\hline
                    \emph{Dependent Variable}:&\multicolumn{6}{c}{Likelihood of Negotiation}\\
                    \cline{2-7}\\ &\multicolumn{1}{c}{(1)}&\multicolumn{1}{c}{(2)}&\multicolumn{1}{c}{(3)}&\multicolumn{1}{c}{(4)}&\multicolumn{1}{c}{(5)}&\multicolumn{1}{c}{(6)}\\
\hline
ln(Issue Size)      &       -0.07         &       -0.06         &       -0.14         &       -0.13         &        0.02         &        0.01         \\
                    &     [-0.55]         &     [-0.50]         &     [-1.00]         &     [-0.97]         &      [0.19]         &      [0.17]         \\
[1em]
ln(avg. bond size)  &        0.13         &        0.12         &        0.17         &        0.17         &        0.01         &        0.02         \\
                    &      [0.92]         &      [0.84]         &      [1.18]         &      [1.13]         &      [0.16]         &      [0.18]         \\
[1em]
Coupon              &        0.05\sym{**} &        0.04\sym{**} &        0.03\sym{**} &        0.03\sym{**} &        0.01         &        0.01         \\
                    &      [2.34]         &      [2.34]         &      [2.04]         &      [2.03]         &      [1.11]         &      [1.11]         \\
[1em]
Maturity            &        0.03         &        0.03         &        0.02         &        0.02         &       -0.02         &       -0.02         \\
                    &      [1.44]         &      [1.29]         &      [1.24]         &      [1.10]         &     [-1.18]         &     [-1.17]         \\
[1em]
Callable            &       -0.06\sym{*}  &       -0.06\sym{**} &       -0.02         &       -0.02         &       -0.02         &       -0.02         \\
                    &     [-1.98]         &     [-2.01]         &     [-0.71]         &     [-0.76]         &     [-0.86]         &     [-0.87]         \\
[1em]
Credit Enh.         &       -0.14\sym{*}  &       -0.14\sym{*}  &       -0.04         &       -0.04         &       -0.00         &       -0.00         \\
                    &     [-1.71]         &     [-1.68]         &     [-0.76]         &     [-0.75]         &     [-0.02]         &     [-0.01]         \\
[1em]
Insured             &        0.10\sym{***}&        0.12\sym{***}&        0.07\sym{**} &        0.08\sym{**} &        0.04         &        0.04         \\
                    &      [2.88]         &      [3.26]         &      [2.35]         &      [2.62]         &      [0.88]         &      [0.89]         \\
[1em]
Bank Qualified      &       -0.10\sym{***}&       -0.09\sym{***}&       -0.05\sym{**} &       -0.04\sym{*}  &        0.01         &        0.01         \\
                    &     [-3.42]         &     [-3.19]         &     [-2.10]         &     [-1.80]         &      [0.92]         &      [1.03]         \\
[1em]
Num. of Bonds       &        0.02         &        0.01         &        0.05         &        0.05         &       -0.00         &       -0.00         \\
                    &      [0.19]         &      [0.17]         &      [0.62]         &      [0.60]         &     [-0.03]         &     [-0.00]         \\
[1em]
GO bond             &                     &       -0.08\sym{**} &                     &       -0.08\sym{**} &                     &       -0.03         \\
                    &                     &     [-2.31]         &                     &     [-2.29]         &                     &     [-0.97]         \\
[1em]
Num. of Txns.       &       -0.04\sym{***}&       -0.04\sym{***}&       -0.03\sym{**} &       -0.03\sym{**} &                     &                     \\
                    &     [-3.09]         &     [-2.78]         &     [-2.39]         &     [-2.25]         &                     &                     \\
[1em]
City(Issuer)        &        0.01         &        0.01         &        0.04         &        0.04         &                     &                     \\
                    &      [0.17]         &      [0.16]         &      [0.95]         &      [0.83]         &                     &                     \\
[1em]
County(Issuer)      &        0.05         &        0.05         &        0.08\sym{**} &        0.09\sym{**} &                     &                     \\
                    &      [1.09]         &      [1.14]         &      [2.08]         &      [2.25]         &                     &                     \\
[1em]
State(Issuer)       &        0.20\sym{***}&        0.18\sym{***}&        0.18\sym{***}&        0.16\sym{***}&                     &                     \\
                    &      [4.26]         &      [3.57]         &      [4.58]         &      [3.90]         &                     &                     \\
[1em]
% Constant            &        0.34\sym{**} &        0.39\sym{**} &        0.19         &        0.24         &        0.33\sym{***}&        0.34\sym{***}\\
%                     &      [2.13]         &      [2.39]         &      [1.20]         &      [1.52]         &      [3.80]         &      [4.47]         \\
\hline
Year FE             &$\checkmark$         &$\checkmark$         &$\checkmark$         &$\checkmark$         &$\checkmark$         &$\checkmark$         \\
Purpose FE          &$\checkmark$         &$\checkmark$         &$\checkmark$         &$\checkmark$         &$\checkmark$         &$\checkmark$         \\
Rating FE           &$\checkmark$         &$\checkmark$         &$\checkmark$         &$\checkmark$         &$\checkmark$         &$\checkmark$         \\
State FE            &                     &                     &$\checkmark$         &$\checkmark$         &                     &                     \\
Issuer FE           &                     &                     &                     &                     &$\checkmark$         &$\checkmark$         \\
Adj.-R$^2$          &       0.174         &       0.178         &       0.307         &       0.311         &       0.686         &       0.686         \\
Obs.                &      15,578         &      15,578         &      15,578         &      15,578         &      15,578         &      15,578         \\
\hline
\end{tabular}
}
\end{table}

\begin{landscape}
\begin{table}[htbp]
\def\sym#1{\ifmmode^{#1}\else\(^{#1}\)\fi}
\caption{Impact on Borrowing Costs of Local Governments: Evidence from  Municipal Bonds Primary Market} 
\label{table:baseline_yld}
\vspace{0.2in}
\par
{\footnotesize This table reports the baseline results for our sample using Equation \eqref{eq:baseline} estimating the differential effect on municipal bond yields of treated and control bonds after the Municipal Advisory Rule of 2014. The primary coefficient of interest, $\beta_0$, is captured by the interaction term of \textit{Treated $\times$ Post}. We show our results using offering yields as the dependent variable. Specifically, Column (1) reports the results without any controls or fixed effects. In Column (2), we first introduce issuer-adviser pair fixed effects. Column (3) shows results by additionally including bond level controls consisting of coupon (\%); log(amount issued in \$); dummies for callable bonds, bond insurance, general obligation bond, bank qualification, and credit enhancement; credit rating; remaining years to maturity; and inverse years to maturity. We provide the description of key variables in Table \ref{table:vardescription}. Column (4) introduces the year fixed effect. In Column (5), we control for the county-level economic conditions. We use the lagged values for log(labor force) and unemployment rate, and the percentage change in unemployment rate and labor force, respectively. Column (6) further introduces the issuer fixed effect, followed by the adviser fixed effect in Column (7). Finally, Column (8) shows results by also adding state-year fixed effects. In Table \ref{table:baseline_yld}, we show our results using offering yields as the dependent variable. T-statistics are reported in brackets and standard errors are clustered at the state level. \sym{*} \(p<0.10\), \sym{**} \(p<0.05\), \sym{***} \(p<0.01\)}\\
% \vspace{.2in}
\vspace{.05in} 
% \resizebox{0.9\textwidth}{!} {

% \raggedright\textbf{Panel A: Primary Market}\\
\vspace{0.1in}
\centering
\resizebox{1.25\textwidth}{!} {
\begin{tabular}{@{\extracolsep{4pt}}l*{8}{c}}
\hline
                    \emph{Dependent Variable}:&\multicolumn{8}{c}{Yield}\\
                    \cline{2-9}\\                    &\multicolumn{1}{c}{(1)}&\multicolumn{1}{c}{(2)}&\multicolumn{1}{c}{(3)}&\multicolumn{1}{c}{(4)}&\multicolumn{1}{c}{(5)}&\multicolumn{1}{c}{(6)}&\multicolumn{1}{c}{(7)}&\multicolumn{1}{c}{(8)}\\
                    % &\multicolumn{3}{c}{Yield}&\multicolumn{3}{c}{Spread}&\multicolumn{3}{c}{yield spread}\\
\hline
Treated $\times$ Post &      -17.98\sym{***}&      -16.23\sym{***}&      -18.59\sym{***}&      -18.53\sym{***}&      -15.21\sym{***}&      -15.21\sym{***}&      -15.21\sym{***}&      -10.55\sym{***}\\
                    &     [-3.82]         &     [-2.92]         &     [-4.18]         &     [-3.57]         &     [-4.38]         &     [-4.38]         &     [-4.38]         &     [-3.61]         \\
[1em]
Treated             &       31.51\sym{***}&       -3.20         &        9.21\sym{*}  &       15.97\sym{***}&       13.57\sym{***}&       13.57\sym{***}&       13.57\sym{***}&       10.56\sym{***}\\
                    &      [4.22]         &     [-0.39]         &      [1.82]         &      [3.58]         &      [4.19]         &      [4.19]         &      [4.19]         &      [3.75]         \\
[1em]
Post                &      -16.61\sym{***}&      -20.36\sym{***}&      -26.05\sym{***}&       -6.46\sym{***}&       -7.03\sym{***}&       -7.03\sym{***}&       -7.03\sym{***}&       -8.40\sym{***}\\
                    &     [-9.52]         &     [-6.47]         &    [-13.11]         &     [-2.90]         &     [-3.68]         &     [-3.68]         &     [-3.68]         &     [-4.96]         \\
[1em]
\hline
Issuer-Adv. FE      &                     &$\checkmark$         &$\checkmark$         &$\checkmark$         &$\checkmark$         &$\checkmark$         &$\checkmark$          &$\checkmark$         \\
Bond Controls       &                     &                     &$\checkmark$         &$\checkmark$         &$\checkmark$         &$\checkmark$         &$\checkmark$         &$\checkmark$         \\
Year FE             &                     &                     &                     &$\checkmark$         &$\checkmark$         &$\checkmark$         &$\checkmark$         &$\checkmark$         \\
County Controls     &                     &                     &                     &                     &$\checkmark$         &$\checkmark$         &$\checkmark$         &$\checkmark$         \\
Issuer FE           &                     &                     &                     &                     &                     &$\checkmark$         &$\checkmark$         &$\checkmark$         \\
Adviser FE          &                     &                     &                     &                     &                     &                     &$\checkmark$         &$\checkmark$         \\
State-Yr. FE        &                     &                     &                     &                     &                     &                     &                     &$\checkmark$         \\
Adj.-R$^2$          &       0.020         &       0.205         &       0.784         &       0.833         &       0.834         &       0.834         &       0.834         &       0.838         \\
Obs.                &     805,013         &     804,764         &     804,764         &     804,764         &     804,764         &     804,764         &     804,764         &     804,764         \\
\hline
\end{tabular}
}
\end{table}
\end{landscape}
\clearpage

\clearpage
\newpage
\begin{table}[htbp]
% \centering
\def\sym#1{\ifmmode^{#1}\else\(^{#1}\)\fi}
% \scriptsize
\caption{Robustness Tests using Offering Yields}
\label{table:robustness_yld}
\vspace{0.2in}
\par
{\footnotesize In this table we report results for various robustness tests on our baseline specification, i.e., Column (8) of Table \ref{table:main_baseline} using offering yield as the dependent variable. Columns (1)-(2) show the baseline effect by changing the dependent variable to after-tax yield and after-tax yield spread, respectively. In Columns (3)-(9), we report results based on alternative econometric specifications. We introduce additional fixed effects to account for unobserved factors that may be varying over time. Specifically, Column (3) reports baseline results by adding issuer-type $\times$ year fixed effects. We add bond purpose $\times$ year fixed effect in Column (4). Columns (5) and (6) show results by adding underwriter fixed effect and underwriter $\times$ year fixed effect, respectively. In Column (7), we add advisor $\times$ year fixed effect. Column (8) reports the baseline result by adding both underwriter $\times$ year fixed effect as well as advisor $\times$ year fixed effect. In Column (9), we replace the issuer-advisor pair fixed effect with the issuer-underwriter pair fixed effect. Columns (10)-(11) show results using a shorter event window. We consider additional tax considerations in Columns (12)-(14). First, we restrict the sample to bonds on which interest income is exempt under federal tax in Column (12). In Column (13), we also omit bonds from five states (IL, IA, KS, OK, WI) that tax interest income on municipal bonds issued in-state or out-of-state \citep{gao2021good}. Column (14) shows results using bonds that are exempt from both state and federal income tax. Columns (15)-(18) report results focusing on sub-samples of homogeneous bonds. Accordingly, in Column (15), we drop bonds in which the advisor and underwriter are same. Column (16) shows results by dropping callable bonds. We drop insured bonds in Column (17). Finally, we focus on only the new money bonds in Column (18). Our results in Columns (19)-(21) focus on additional geographic considerations. We keep only local bonds (by dropping state level bonds) in Column (19). Conversely, we show results using only the state level bonds in Column (20). In Column (21), we report the baseline results by dropping issuances from the three largest municipal bond issuers, namely: California, New York and Texas. We consider alternative levels of clustering standard errors in Columns (22)-(32). In Columns (22)-(25), we cluster standard errors by advisor, issuer, issuer(2), and bond issue, respectively. Issuer(2) refers to weakly identifying borrowers based on the first six-digits of the bond CUSIP \citep{gao2021good}. Columns (26)-(28) double cluster standard errors along two dimensions in the cross section: state-advisor, advisor-underwriter, and advisor-issuer, respectively. Finally, in Columns (29)-(32), we double cluster standard errors over time and across bonds using: state and year, advisor and year, state and year-month, and advisor and year-month, respectively. T-statistics are reported in brackets and standard errors are clustered at the state level, unless otherwise specified. \sym{*} \(p<0.10\), \sym{**} \(p<0.05\), \sym{***} \(p<0.01\)}\\
\end{table}
\clearpage
\newpage
\begin{landscape}
\begin{table}
    \centering
    \def\sym#1{\ifmmode^{#1}\else\(^{#1}\)\fi}
    \vspace{0.2cm}
    \resizebox{1.3\textwidth}{!}{
\begin{tabular}{@{\extracolsep{4pt}}l*{11}{c}@{}}
\hline
                    \emph{Dependent Variable}: &\multicolumn{11}{c}{Offering Yield (basis points)} \vspace{0.2in} \\
                    &\multicolumn{2}{c}{Other Dependent Variables}&\multicolumn{7}{c}{Alternative Specifications}&\multicolumn{2}{c}{Shorter Event Window}\\
                    \cline{2-3} \cline{4-10} \cline{11-12} \\
                    &\multicolumn{1}{c}{After-tax  }&\multicolumn{1}{c}{After-tax }&\multicolumn{1}{c}{Add Issuer-Type}&\multicolumn{1}{c}{Add Purpose}&\multicolumn{1}{c}{Add }&\multicolumn{1}{c}{Add }&\multicolumn{1}{c}{Add }&\multicolumn{1}{c}{Add Adv.-Yr. }&\multicolumn{1}{c}{Use }&\multicolumn{1}{c}{2014-2017}&\multicolumn{1}{c}{2013-2016}\\                   &\multicolumn{1}{c}{Yield}&\multicolumn{1}{c}{Yield Spread}&\multicolumn{1}{c}{Year FE}&\multicolumn{1}{c}{Year FE}&\multicolumn{1}{c}{UW FE}&\multicolumn{1}{c}{UW-Yr. FE}&\multicolumn{1}{c}{Adv.-Yr. FE}&\multicolumn{1}{c}{and UW-Yr. FE}&\multicolumn{1}{c}{Issuer-UW FE}&\multicolumn{1}{c}{}&\multicolumn{1}{c}{}\\ &\multicolumn{1}{c}{(1)}&\multicolumn{1}{c}{(2)}&\multicolumn{1}{c}{(3)}&\multicolumn{1}{c}{(4)}&\multicolumn{1}{c}{(5)}&\multicolumn{1}{c}{(6)}&\multicolumn{1}{c}{(7)}&\multicolumn{1}{c}{(8)}&\multicolumn{1}{c}{(9)}&\multicolumn{1}{c}{(10)}&\multicolumn{1}{c}{(11)}\\
\hline\\
\vspace{0.2cm}
Treated $\times$ Post &      -17.20\sym{***}&      -19.91\sym{***}&      -10.33\sym{***}&       -9.97\sym{***}&      -10.95\sym{***}&      -10.15\sym{***}&       -8.16\sym{***}&       -8.34\sym{***}&      -10.54\sym{***}&       -6.19\sym{*}  &       -8.96\sym{***}\\
                    &     [-3.67]         &     [-4.19]         &     [-3.56]         &     [-3.47]         &     [-4.22]         &     [-3.64]         &     [-2.76]         &     [-3.03]         &     [-2.81]         &     [-1.84]         &     [-3.57]         \\
[1em]
Adj.-R$^2$          &       0.837         &       0.828         &       0.838         &       0.838         &       0.840         &       0.842         &       0.844         &       0.847         &       0.868         &       0.881         &       0.877         \\
Obs.                &     803,112         &     802,426         &     803,506         &     803,517         &     803,876         &     803,867         &     804,755         &     803,858         &     804,110         &     346,091         &     333,795         \\
\hline
\end{tabular}
}\\

% \vspace{1cm}
\medskip
% \vspace{-2em}
   \resizebox{1.3\textwidth}{!}{
\begin{tabular}{@{\extracolsep{4pt}}l*{10}{c}@{}}

                    \emph{Dependent Variable}: &\multicolumn{10}{c}{Offering Yield (basis points)} \vspace{0.2in}\\
                    \cline{2-11} \\
                    &\multicolumn{3}{c}{Tax Considerations}&\multicolumn{4}{c}{Bond Considerations}&\multicolumn{3}{c}{Geographic Considerations}\\
                    \cline{2-4}  \cline{5-8} \cline{9-11} \\ &\multicolumn{1}{c}{Exempt}&\multicolumn{1}{c}{Drop non-}&\multicolumn{1}{c}{Exempt}&\multicolumn{1}{c}{Drop same}&\multicolumn{1}{c}{Drop}&\multicolumn{1}{c}{Drop}&\multicolumn{1}{c}{Only}&\multicolumn{1}{c}{Keep}&\multicolumn{1}{c}{Keep}&\multicolumn{1}{c}{Drop}\\       &\multicolumn{1}{c}{(Federal)}&\multicolumn{1}{c}{Exempt States}&\multicolumn{1}{c}{(Fed.+State)}&\multicolumn{1}{c}{Adv.-UW. bonds}&\multicolumn{1}{c}{Callable}&\multicolumn{1}{c}{Insured}&\multicolumn{1}{c}{New money}&\multicolumn{1}{c}{Local}&\multicolumn{1}{c}{State}&\multicolumn{1}{c}{CA,NY,TX}\\                    &\multicolumn{1}{c}{(12)}&\multicolumn{1}{c}{(13)}&\multicolumn{1}{c}{(14)}&\multicolumn{1}{c}{(15)}&\multicolumn{1}{c}{(16)}&\multicolumn{1}{c}{(17)}&\multicolumn{1}{c}{(18)}&\multicolumn{1}{c}{(19)}&\multicolumn{1}{c}{(20)}&\multicolumn{1}{c}{(21)}\\
\hline\\
\vspace{0.2cm}
Treated $\times$ Post &      -11.04\sym{***}&       -9.67\sym{***}&      -10.13\sym{***}&      -10.53\sym{***}&      -11.50\sym{***}&      -12.29\sym{***}&      -20.49\sym{***}&       -9.20\sym{***}&      -13.45\sym{***}&      -14.84\sym{***}\\
                    &     [-3.35]         &     [-2.95]         &     [-3.10]         &     [-3.64]         &     [-5.72]         &     [-5.33]         &     [-4.50]         &     [-2.88]         &     [-2.94]         &     [-7.25]         \\
[1em]
Adj.-R$^2$          &       0.868         &       0.866         &       0.866         &       0.838         &       0.802         &       0.838         &       0.857         &       0.848         &       0.782         &       0.842         \\
Obs.                &     739,157         &     663,786         &     686,692         &     801,245         &     442,138         &     663,644         &     395,925         &     715,364         &      89,397         &     516,019         \\
\hline
\end{tabular}
}\\

% \vspace{1cm}
% \vspace{-2em}
\medskip
   \resizebox{1.3\textwidth}{!}{
\begin{tabular}{@{\extracolsep{4pt}}l*{11}{c}@{}}
                    \emph{Dependent Variable}: &\multicolumn{11}{c}{Offering Yield (basis points)} \vspace{0.2in} \\
                    \cline{2-12} \\
                    &\multicolumn{11}{c}{Alternative Clustering}\\
                    \cline{2-12}\\                    &\multicolumn{1}{c}{Advisor}&\multicolumn{1}{c}{Issuer}&\multicolumn{1}{c}{Issuer(2)}&\multicolumn{1}{c}{Issue}&\multicolumn{1}{c}{State, Advisor}&\multicolumn{1}{c}{Advisor, UW}&\multicolumn{1}{c}{Advisor, Issuer}&\multicolumn{1}{c}{State, Year}&\multicolumn{1}{c}{Advisor, Year}&\multicolumn{1}{c}{State, YM}&\multicolumn{1}{c}{Advisor, YM}\\    &\multicolumn{1}{c}{(22)}&\multicolumn{1}{c}{(23)}&\multicolumn{1}{c}{(24)}&\multicolumn{1}{c}{(25)}&\multicolumn{1}{c}{(26)}&\multicolumn{1}{c}{(27)}&\multicolumn{1}{c}{(28)}&\multicolumn{1}{c}{(29)}&\multicolumn{1}{c}{(30)}&\multicolumn{1}{c}{(31)}&\multicolumn{1}{c}{(32)}\\
\hline\\
\vspace{0.2cm}
Treated $\times$ Post &      -10.55\sym{***}&      -10.55\sym{***}&      -10.55\sym{***}&      -10.55\sym{***}&      -10.55\sym{***}&      -10.67\sym{***}&      -10.55\sym{***}&      -10.55\sym{***}&      -10.55\sym{***}&      -10.55\sym{***}&      -10.55\sym{***}\\
                    &     [-4.45]         &     [-6.97]         &     [-8.42]         &     [-9.94]         &     [-3.30]         &     [-4.30]         &     [-4.35]         &     [-3.45]         &     [-4.05]         &     [-3.65]         &     [-4.48]         \\
[1em]
Adj.-R$^2$          &       0.835         &       0.835         &       0.838         &       0.838         &       0.835         &       0.835         &       0.835         &       0.838         &       0.835         &       0.838         &       0.835         \\
Obs.                &     804,764         &     804,764         &     804,764         &     804,764         &     804,764         &     803,880         &     804,764         &     804,764         &     804,764         &     804,764         &     804,764         \\
\hline
\end{tabular}
}
\end{table}
\end{landscape}
