# Supplementary material for: Fiduciary Duty in the Municipal Bonds Market
Source: arXiv:2406.15197 source file (2024-06-21)
Supplement: Supplementary file 2 [file Appendix_PLOS.tex]

\setcounter{table}{0}
\setcounter{page}{0}

\setcounter{figure}{0}

\setcounter{section}{0}
\setcounter{equation}{0}

\clearpage
% \linespread{0.8}
\doublespacing

\section{SEC Municipal Advisor Rule}\label{sec:sec_ma_rule}
As shown in Figure \ref{fig:total_iss}, municipalities issue over USD 400 billion of municipal bonds each year to finance various infrastructure and public utility projects. However, these municipalities may often lack the financial sophistication to navigate the issuance process \citep{garrett2021conflicts}. Under the Congressional mandate of June 1975, the MSRB has been charged with protecting investors to prevent fraud and financial irregularities in the municpial bond market\footnote{\href{https://www.msrb.org/About-MSRB/About-the-MSRB/Creation-of-the-MSRB.aspx}{https://www.msrb.org/About-MSRB/About-the-MSRB/Creation-of-the-MSRB.aspx}}. Following the financial crisis of 2007-09, Congress passed the Dodd-Frank Wall Street Reform and Consumer Protection Act in 2010. This Act introduced major changes to the regulatory framework and operations of the financial service industry. It also included several provisions concerning SEC rulemaking.
% As a result, the process of issuing municipal bonds in the United States has been monitored by the Municipal Securities Rulemaking Board (MSRB), which develops rules on how financial services firms deal with issuers.

Under this framework, the SEC drew up the Municipal Advisor Rule which became effective on July 1, 2014. Specifically, it became unlawful for a municipal advisor (MA) to provide advice to or on behalf of a municipal entity or obligated person with respect to municipal financial products or the issuance of municipal securities unless the MA is registered with the SEC. Prior to this reform, only broker-dealers and banks were subject to federal regulatory requirements. The SEC sought to mitigate some of the problems observed in the conduct of municipal advisors in the municipal bond market. This included the municipal advisor's failure to place the duty of loyalty to their clients ahead of their own interests \citep{white2014}. Additionally, the SEC Commissioner noted in a statement in 2013\footnote{\href{https://www.sec.gov/news/statement/2013-09-18-open-meeting-statement-kms}{https://www.sec.gov/news/statement/2013-09-18-open-meeting-statement-kms}}:
\vspace{-1em}
\begin{verse}
\noindent
\textit{Our dedicated public servants were relying on municipal advisors whose advisory activities generally did not require them to register with the Commission, or any other federal, state, or self-regulatory entity.    And a lack of meaningful regulation over these advisors created confusion, and in some instances, horrific abuses.  Sadly, the shortcomings of this hands-off regulatory regime became glaringly apparent during the last several years as we learned about numerous examples of bad behavior, including self-dealing and excessive fees.}
\end{verse}

Importantly, advisors owe fiduciary responsibility to municipal clients under the MA Rule and cannot act in ways that my be unfavorable to their clients. This would encompass the twin requirements of duty of care, and duty of loyalty. According to the former, advisors must exert effort on behalf of the issuer in order to make a recommendation. The duty of loyalty requires advisors to uphold the interests of the issuer superior to their own. Failing to adhere to their fiduciary responsibility, advisors may be held liable for adverse outcomes to issuers during municipal bond issuance. The SEC MA Rule also clarified what constitutes municipal advice and therefore under what circumstances the registration requirements would be applicable. Broadly, the SEC documented ``advice'' as any recommendation particularized to specific needs, objectives, and circumstances of a municipal entity. Overall, the SEC Municipal Advisor Rule introduced a new set of standards applicable to municipal advisors, with an aim to help municipal issuers.

\section{Advisor Names}\label{sec:adv_names}
There is substantial variation in the names used by FTSE Russell municipal bond database to record municipal advisors involved in the issuance of bonds. Often these variations are due to spellings like ``BACKSTORM MCCARLEY BERRY \& COMPANY LLC'' vs ``BACKSTROM MCCARLEY BERRY \& COMPANY''. I investigate the bond offer statement associated with the CUSIP to verify the corresponding entity and update the standardized name. Besides the jumbled spelling errors, I also come across typos and mistakes due to omitted letters. For example, ``BERKSHIRE BANK'' and ``BERSHIRE BANK'' correspond to the same municipal advisor. Further, I also account for alternative company name extensions, such as, ``LLC'', ``INC'', ``Co.'' or ``CO.''. These extensions are recorded differently over time for the same company. Occasionally, the names would omit portions of the names altogether: ``SUDSINA \& ASSOCIATES'' was also reported as ``SUDSINA''. To verify against mismatching firm names, I rely on logos printed on the bond's offering statement in addition to the official address provided. 
% The address typically includes the name of the city and state.

Other instances of spelling differences involve special characters like ``.'' or ``,'' and ``\&''. Clearly, these are easy to handle and to resolve. I also need to update names for subsidiaries and affiliated company names. These would also often involve mergers and acquisitions. Following \cite{cestau2020specialization}, I retroactively replace the names of the merged entities with the name of the new company. To an extent, this assumes that client relationships prevailed even after the M\&A activity. Indeed I do find evidence where both sets of names are found in the offering statements. This could also be due to delay in sale of bonds, especially via negotiation. Thus, offer statements may reflect contractual engagements before or after the merger activity. As a result, I identify these entities under a common name: for example, ``MERRILL LYNCH \& COMPANY'' and ``BANC OF AMERICA SECURITIES'' as ``BANC OF AMERICA SECURITIES''. I also find limited anecdotal evidence suggesting that acquisitions involve retention of officials in the new company.

Still other challenges include names where firms operate using different brand names. For example, ``SUSAN D. MUSSELMAN INC'', ``SDM ADVISORS INC'' and ``DASHENMUSSELMAN INC'' are captured differently. However, I represent them as ``A DASHEN \& ASSOCIATES'' by checking the names of principals and office locations recorded under each company. I believe that it is very difficult to identify abbreviated names corresponding to the same umbrella company without verifying each name separately. In some cases, I need to ascertain the office locations from internet search versus that reported in the bond offering statement. But I also come across simpler associations where alternative trading names used by companies are seemingly related, such as, ``RV NORENE \& ASSOCIATE INC'' and ``CROWE NORENE''. 

\section{\label{subsec:selecting_nego}Threats to Identification}
An obvious concern with the identification strategy above relates to selection. Issuers that choose to raise municipal debt via negotiation may be different from those who do not. In order to test whether selection may likely bias the estimates of a difference-in-differences design, I evaluate the type of issuers who choose negotiation. I estimate a linear probability regression describing the choice of selling bonds via negotiation (indicator $\mathbbm{1}\{Nego._{b,i,t}$) as,
\begin{equation}\label{eq:like_nego}
 \mathbbm{1}\{Nego._{b,i,t}=1\} = \kappa_{t} + \beta*X_{b,i,t} + \epsilon_{b,i,t}       
\end{equation}
where subscript $b$ indicates the bond issuance, $i$ indicates the issuer, and $t$ indicates the time. $X_{b,i,t}$ includes variables controlling for issue size, average bond size, coupon, years to maturity, callable status, credit enhancement, insurance status, bank qualification, number of bonds, type of security (general obligation vs revenue), type of issuer, frequency of issuer borrowing, and fixed effects for rating group as well as use of funds (bond purpose). 

I estimate this regression over three approaches to demonstrate how various factors affect the choice of negotiation. I focus on the three years before the SEC Municipal Advisor Rule to capture the ex-ante snapshot. Figure \ref{fig:like_nego} shows the estimated coefficients for each specification using bond issuances for the three years before the SEC Municipal Advisor Rule. I also provide the tabular results in Table \ref{table:like_nego}. First, I show results from the \emph{Overall} balance without using any geographic controls. The results suggest that there is some variation in terms of using negotiated sale for bonds that are insured as well as for state level bonds. Certain bonds that need outside insurance from a third-party may be well suited for sale via negotiation. At the same time, state level issuers may be better suited for negotiation given their previous relationships \citep*{brown2017politics}. When I include state fixed effects (\emph{Within State}), I find similar factors driving the choice of negotiation. 

However, importantly for identification here, these differences get wiped out when I consider the variation after including issuer fixed effects (\emph{Within Issuer}). In this specification, I capture the likelihood of negotiation among issuers who borrow multiple times choosing negotiated or competitive sale for different issues. My strategy in Equation \eqref{eq:baseline} looks to compare issuer-advisor pairs that sell bonds using negotiated versus competitive auction of bonds. By showing that issue characteristics do not seem to affect the choice of negotiation within issuers, I provide support against ex-ante selection concerns. Moreover, I also depict the portion of advised bonds sold via negotiation and competitive bidding in Figure \ref{fig:amt_nego}. I do not find evidence for changing method of sale around the Municipal Advisor Rule. Nearly 40\% of the bond volume is consistently sold via negotiation around 2014. I also show this more formally in Figure \ref{fig:ll_nego} by plotting the coefficients from regressing the likelihood of negotiation on half-year dummies after including issuer fixed effects. Benchmarked to the period before the Rule, I do not find any statistical difference around the SEC Rule. This evidence helps against concerns about selection into negotiation over time.

\section{\label{subsec:robustness}Robustness}
In this section, I test the robustness of the main result in Column (8) of Table \ref{table:main_baseline} to various alternative econometric considerations. I present the results of these robustness checks in Table \ref{table:robustness} ranging across different dependent variables, alternative specifications, tax and bond considerations,  geographic considerations as well as alternative clustering of standard errors. 

\subsection{Other Dependent Variables}\noindent
To show robustness of the main result to the choice of dependent variable, I show the results using after-tax yield (Column (1)) and after-tax yield spread (Column (2)). The construction of the tax-adjusted yield spread follows \citet*{schwert2017municipal}. I describe these variables in Table \ref{table:vardescription}. I find the main coefficient to be statistically significant with magnitudes of -18.13 bps and -19.69 bps, respectively. These higher magnitudes are not surprising because the tax adjustment tends to scale up the yields, as also shown in \citet*{gao2021good}. I also replicate the baseline table using offering yield as the dependent variable. Specifically, Column (8) in Table \ref{table:baseline_yld} corresponds to the main specification. I conclude that the main result is not sensitive to the specific choice of dependent variable.

There may be a concern that since municipal bonds are generally issued in a series \citep*{ang2017advance}, their pricing should be evaluated as a package. Ideally, the total interest cost may be a measure of such issue-level bond package. However, the FTSE Russell municipal bond database does not capture this variable. To overcome this limitation, I proceed by taking a weighted average of the yields across bonds in a given series/package. Similarly, I also aggregate the bond level characteristics across bonds in the same package to arrive at issue-level characteristics. Figure \ref{fig:did_issuYield} shows the baseline result in a dynamic regression \emph{within} issuers. I quantify the baseline magnitude using this definition of issue-level yields and issue-level yield spreads in Table \ref{table:issu_yld} and Table \ref{table:issu_spread}, respectively. The preferred specification is shown in Column (8), where the magnitude looks similar to the main analysis and is statistically significant. Therefore, I conclude that the main specification is robust to this alternative consideration of measuring the main dependent variable.

\subsection{Alternative Specifications}\label{subsubsec:alt_spec}\noindent
In Column (3), I show the baseline results by adding issuer-type $\times$ year fixed effects. By augmenting the model, I add flexible time trends for different types of issuers (city, county, state or other) interacted with year fixed effects. There may be a concern that municipal advisors specialize in the type of local governments they advise that may change around the same time as the SEC Municipal Advisor Rule. I attempt to absorb how such secular trends may unobservably affect different types of issuers. I find that the coefficient of interest is statistically significant and close to the baseline value.

Municipal bonds are issued with the objective of funding or financing specific types of projects/objectives. These could range from activities pertaining to infrastructure (like schools, highways, water-sewer), general purpose and public improvement, or servicing existing utilities like power generation. Each of these sub-markets may experience differences in underlying risks associated with bonds raised for that purpose. As a result, I show results after controlling for the underlying purpose of bonds in Column (4). I also control for such unobserved trends over time by including bond purpose $\times$ year fixed effects in Column (5). I find that the magnitude (-12.19 bps) is nearly similar to the main effect and is statistically significant. Thus, I rule out explanations about the main effect that may be linked to trends in the purpose of bonds which may change around the same time as the imposition of fiduciary duty.

\citet*{cestau2020specialization} shows that underwriters tend to specialize in the method of sale in the municipal bond market. Moreover, \citet*{cestau2019competition} also argues that market concentration has increased in municipal bond underwriting, especially due to negotiated sales. In light of this, I address the possibility that unobserved changes among underwriters may simultaneously affect yields as the SEC Municipal Advisor Rule. First, in Column (6), I include underwriter fixed effects to the main specification to absorb unobserved characteristics across underwriters. I find the interaction coefficient of \textit{Treated $\times$ Post} to be -12.92 bps and statistically significant. Further, I also absorb unobserved time-varying trends associated with underwriters (underwriter $\times$ year fixed effects) and present the results in Column (7). The reported coefficient is -11.07 bps. Overall, I argue that the results are robust to unobserved time-unvarying and time-varying changes related to underwriters.

There may be a concern that issuers and advisors may rely on past relationships during new municipal bond issuances. This may allow advisors to gather more information about issuers with whom they work repeatedly. I account for this unobserved effect by including issuer-advisor pair fixed effect in Column (8), and find that the main result is robust to this consideration. Alternatively, one may argue that a similar alignment between issuers and underwriters may be driving the lower yields. Once again, I address this concern by introducing issuer-underwriter pair fixed effect to the main specification. Column (9) shows that the estimate is similar (-14.20 bps) after accounting for this. overall, I show that unobserved factors driving issuer-advisor and issuer-underwriter relationships do not drive the main result.

Besides the issuer-advisor relationship discussed above, advisors may be specializing over specific states. For example, Panel A Table \ref{table:summary_bonds1} reports that most advisors among the top 15 operate over multiple states. However, over 50 percentile of the bond volume advised by them may come from less than ten states. In light of this, I examine the sensitivity of the baseline result to controlling for unobserved advisor-state pairing. Column (10) shows that the baseline effect is robust to this consideration. Finally, I also show results for a restrictive specification in Column (11), by including county $\times$ year fixed effect. Offering yield spreads may be unobservably driven by local economic conditions at the county level. This accounts for any unobserved time-varying heterogeneity among issuers for the county in which they belong. For state-issued bonds, this corresponds to the state $\times$ year fixed effect in the data. Even with this granular fixed effect, I find that the main coefficient is only slightly lower (-10.65 bps) and remains statistically significant. 

\subsection{Additional Considerations on Taxability, Bond features and Geography}\noindent
An attractive feature of the municipal bond market is that interest income from most bonds is exempt from federal and state taxes \citep{green1993simple,schwert2017municipal}. This greatly appeals to investors who fall in the high income tax bracket. \cite{landoni2018tax} discusses the effects of tax distortions in interest income in municipal bond pricing. Given the heterogeneous effects due to tax considerations, I also show robustness of the main results to these aspects in Columns (12)-(14). First, in Column (12), I broaden the sample to bonds for which interest income is taxable under federal law. I find the effect to be -11.93 bps and statistically significant. Next, I drop bonds from states that do not provide income tax exemption for in-state or out-of-state municipal bonds (IL, IA, KS, OK, WI)  \citep*{gao2021good}. Here, I report a baseline estimate of -11.08 bps in Column (13). Finally, I only focus on bonds that are exempt from federal as well as state level taxes in Column (14). The reported coefficient is -11.94 bps and is statistically significant. Thus, I conclude that the results are not sensitive to these tax considerations on interest income from municipal bonds.

For the baseline analysis, I present the results using a wide variety of municipal bonds. These may vary in terms of the purpose (and I show robustness in Section \ref{subsubsec:alt_spec}) or type of bond features \citep*{brancaccio2021search}. These aspects may also drive and govern the advisors and underwriters that are associated with the bonds at the time of sale. For example, bonds that are advised and underwritten by the same financial agent may be unobservably different and may confound the estimates. However, in Column (15) of Table \ref{table:robustness}, I show the results by dropping a small number of such bonds during the sample period and find a similar effect. Another frequent feature in this market involves callability of the bonds. \citet*{chen2022calling} show that municipalities lose money due to delays in refinancing their callable debt. To the extent that yields may vary unobservably differently for callable bonds around the same time as the SEC regulation, the estimates may be confounded. As a result, I show the baseline effect by dropping callable bonds in Column (16) and show that the findings are robust. Owing to similar considerations of unobserved heterogeneity, I also show results by dropping insured bonds (in Column (17)) and keeping only new money bonds (in Column (18)), respectively. I find that the baseline magnitude increases for these sub-samples and remains statistically significant.

Finally, I turn to geographic considerations that may confound with the identification strategy. In this regard, one may worry that there is substantial heterogeneity in respect of the size and type of issuers. While I also address some of these concerns in Section \ref{subsubsec:alt_spec} by including issuer-type $\times$ year fixed effects, I revisit this aspect here. First, local bonds may be different from state level bonds/issuers. As a result, I show the result by keeping only local bonds in Column (19), followed by restricting the sample to state level bonds only in Column (20). While the magnitude reduces marginally to -10.81 bps in the former, I find a greater impact (-17.15 bps) for state level bonds. The greater effect on state bonds is consistent with the higher impact on more sophisticated issuers, discussed in Section \ref{subsec:hetero_sophis}. Next, I also address any concerns about the relative proportion of municipal bonds issued by different states. The states with the largest municipal debt issuance are California, New York and Texas. I show the robustness of the analysis by dropping observations from these states in Column (21) to show that the results are not driven by these states alone. 

\subsection{Alternative Clustering of Standard Errors}\noindent
I follow a conservative approach in clustering standard errors by state in the baseline specification. However, one may worry that there might be correlation along other dimensions in municipal bond yields, for example, among advisors. In this regard, I consider alternative levels of clustering standard errors in Columns (22)-(32). First, I think of modifying the cross-sectional dimension of observations. In Column (22), I cluster standard errors by advisor and find the main result holds. The baseline effect is also robust to clustering standard errors by underwriters (Column (23)). Column (24) shows results by clustering standard errors by issuer. I also consider a weaker definition to identify issuers based on first six digits of the CUSIP and report the results in Column (25). The results also hold when I cluster by bond issue (Column (26)).

Next, I look to double cluster standard errors along two dimensions. If standard errors in yields are simultaneously correlated with state and advisor, I present results in Column (27) by double clustering errors. Likewise, I show results for clustering by advisor and issuer (Column (28)). Further, I shows robustness of the results to alternative specification involving double clustered standard errors along the cross-section and over time. Specifically, I double cluster by state and year in Column (29), and by advisor and year in Column (30). Finally, I modify the time dimension of clustering to year-month and report the results based on double clustering by state and year-month in Column (31), followed by advisor and year-month in Column (32). In all these specifications, the baseline result holds at the conventional levels of statistical significance, suggesting that the findings are robust to these alternative considerations of clustering standard errors.

Overall, I perform several robustness checks for the baseline specification and find that the main result is not driven by these alternative considerations/explanations. I show that the effect holds even after additional fixed effects, or stricter requirements involving smaller sub-samples or other dependent variables. Moreover, I find similar results by using alternative approaches to clustering standard errors. These evidence enhance the argument of a causal interpretation of the main result in the paper. In Table \ref{table:robustness_yld}, I replicate these analyses using offering yields as the dependent variable. The results suggest that the main effect continues to be robust and significant across these alternative considerations. Finally, I perform similar evaluation using offering price as the dependent variable and report the results in Table \ref{table:robustness_offPrice}.

\section{\label{subsec:refunding}Evidence from Municipal Bond Refundings}
Since the late 1990s, there has been an increasing trend of municipal bond issuance associated with refunding transactions \citep*{ang2017advance}. More specifically, advance refundings allow municipalities to retire an existing callable bond to before its call date \citep{moldogaziev2012state,luby2012use}. Refunding bonds are used to refinance existing municipal debt. Previous evidence in the literature points toward compromised option value \citep{damon1993note}, and the timing of advance refundings \citep*{kalotay1998timing}. In their analysis using an extensive data set, \citet*{ang2017advance} find that a substantial number of advance refundings occur at a net present value loss. They explain their results based on financial constraints of issuers. Given that refundings constitute a large portion of debt in the municipal bond market, I shed light on these issuances in light of fiduciary duty on advisors.

I begin the analysis by first restricting the sample to bonds issued for the purpose of refundings. This allows me to isolate the impact of fiduciary duty by replicating the baseline Equation \eqref{eq:baseline} for a relatively homogeneous group of bonds. Figure \ref{fig:REF_spread} shows the dynamic coefficients obtained from Equation \eqref{eq:dyn_yield_CompNego} for the subset of refunding bonds. In Panel (a), I plot the coefficients on yield spreads over time and find justification for the parallel trends assumption in the period before the SEC Municipal Advisor Rule. Following the imposition of the fiduciary duty on advisors, I find that bond yields decrease for the treated bonds. Compared to the control group, this difference is statistically significant, as shown in Panel (b) of Figure \ref{fig:REF_spread}. For the period before the Rule, I are able to verify that the differences are indistinguishable from zero and statistically insignificant.

To quantify the overall magnitude on yield spreads of bond refundings, I present the results in Table \ref{table:refunding}. Using the offering yields as the dependent variable in the full model specification of Equation \eqref{eq:baseline} in Column (1), I find that yields decrease by 7.93 basis points for the treated bonds. In Column (2), I show the results using the after-tax yield as the dependent variable. As expected, the coefficient of interest is higher, given the tax-adjustments. The baseline specification corresponds to Column (3), where I show results for yield spreads as the dependent variable. I find that refunding yield spreads decrease by 7.54 bps for negotiated bonds after the SEC Municipal Advisor Rule, in comparison to competitively bid bonds. Finally, I also report the results using after-tax yield spreads as the dependent variable in Column (4). As in shown in Column (2), this effect tends to be higher due to tax adjustments (see \citet*{gao2021good}). Overall, I find that the reduction in yields of treated bonds is lower for refunding bonds, when compared to the overall sample. This should be understood in light of the greater information that issuers have about these bonds. Since refundings are issued to refinance earlier bonds, issuers have more information about the underlying characteristics and finances of these projects/purposes. Further, issuers may learn about the demand for such bonds based on the secondary market trading of existing bonds to be refinanced. Thus, the principal-agent problem mitigated by the imposition of fiduciary duty is relatively lower in this setting.

Finally, I turn to another aspect of refunding bond issuances. \citet*{chen2022calling} show that many local governments refinance their long-term debt with significant delays. This results in sizable losses for these issuers. Motivated by this evidence, I examine the timing of pre-refunding bonds in the sample. For these bonds, issuers raise the refunding bonds before the calling date of the bonds to be defeased. Ideally, issuers would benefit the most when such callable bonds are refinanced when they can borrow at the lowest yields. However, the future borrowing cost of issuers may not be precisely ascertained in advance.

The imposition of fiduciary duty on municipal advisors may hold them liable for adverse consequences to municipal issuers. Advisors may be more cautious in issuing refunding bonds in advance of the calling date. I examine this possibility using Equation \eqref{eq:dyn_yield_CompNego} in Figure \ref{fig:timing_refunding_typeL} with the gap between calling date and refunding date as the dependent variable. First, panel (a) shows that the treated and control bonds seem to follow nearly parallel trends \emph{within} issuers. As before, I plot the difference between the treated and control bonds along with the confidence intervals in Figure \ref{fig:timing_ref_diff}. These results show that the gap reduced significantly for the negotiated bonds in the period after the SEC Municipal Advisor Rule. This would suggest that issuers reduced earlier refunding of callable bonds after the imposition of fiduciary duty on their advisors. 

I present this result more formally to quantify the magnitude in Table \ref{table:timing_refunding_typeL}. The preferred specification corresponds to Column (5) where the dependent variable is the gap between the calling and refunding dates. The coefficient suggests that this gap reduced by nearly 143 days, \emph{within} issuers, after controlling for advisor fixed effect and state $\times$ year fixed effect. Due to the smaller sample in this setting, I do not use the more restrictive advisor $\times$ year fixed effect in this setting. Finally, Column (6) shows the result by using the log transformation of the gap in days, suggesting over 20\% reduction for the treated bonds after the SEC Municipal Advisor Rule.

Overall, I show in this Section that there is a similar impact on yield spreads of treated bonds among refunding issuances. Focusing on these bonds also enables understanding more about how issuers reduce the extent of early refunding of callable bonds. These findings complement the main result showing that the imposition of fiduciary duty may benefit the average issuer by lowering their yield spreads at issuance.

\clearpage
\linespread{0.4}
	\newpage {\footnotesize
		\putbib
		}

\clearpage
    \newpage
    
\begin{figure}
\begin{center}
\textbf{Quantile-quantile plot of bond characteristics}
\end{center}
\centering
\includegraphics[scale=0.8]{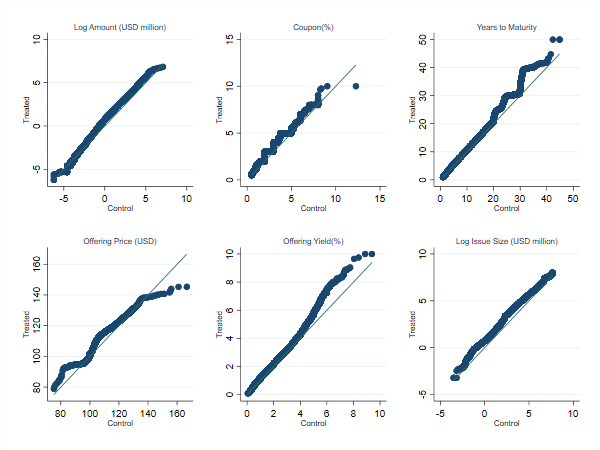}
% \label{fig:muni_adv_fees}

\caption{\footnotesize{The figure shows the primary market characteristics of bonds with advisors at the time of issuance, using a quantile-quantile plot. In my setting, bonds sold via negotiation consist of the ``treated'' group, whereas competitively auctioned bonds comprise the ``control'' group. I focus on fixed rate, tax-exempt bonds issued during 2010-2019.}}
\label{fig:qq_chars}
\end{figure}
    
\begin{figure}
\begin{center}
\textbf{Total Issuance: Negotiated vs Competitive}
\end{center}
\centering
\includegraphics[scale=0.85]{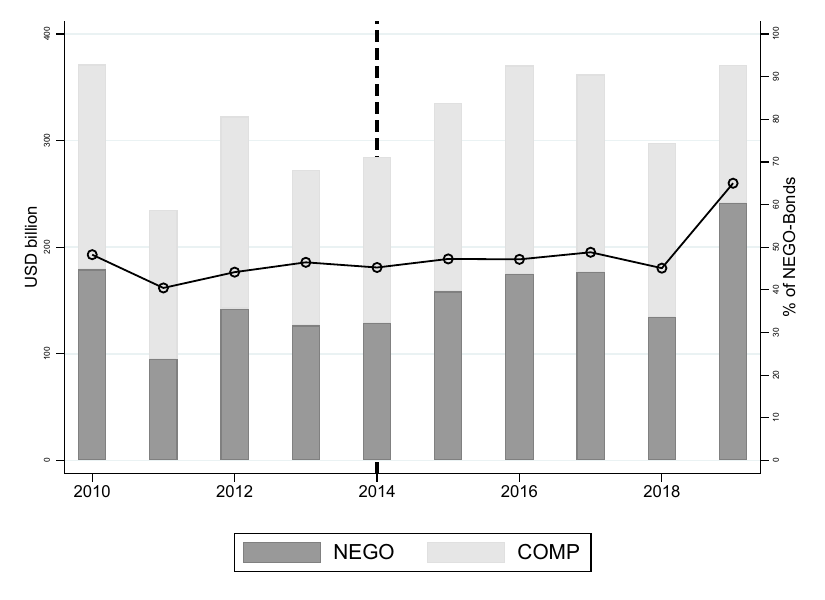}

\caption{\footnotesize{This figure shows the annual amount of advised bonds sold via negotiation. The left hand axis corresponds to the vertical bars denoting the amounts in USD billion. The line graph represents the percentage of dollar value sold via negotiation, shown on the right axis.}}
\label{fig:amt_nego}
\end{figure}

\begin{figure}
\begin{center}
\textbf{Likelihood of Negotiated Sale}
\end{center}
\centering
\includegraphics[scale=0.85]{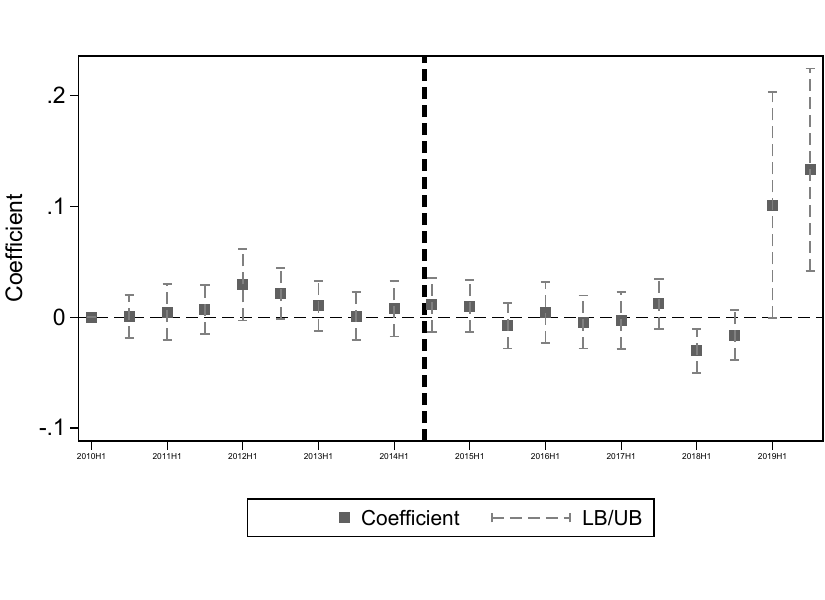}

\caption{\footnotesize{This figure reports the likelihood of issuing a bond via negotiation, \textit{within} issuer. The coefficients are shown relative to a benchmark period of half year period at the start of the event window. Standard errors are clustered at the state level.}}
\label{fig:ll_nego}
\end{figure}

\begin{figure}
\begin{center}
\textbf{Raw Binscatter of Offering Yields}
\end{center}
\centering
\includegraphics[scale=1.2]{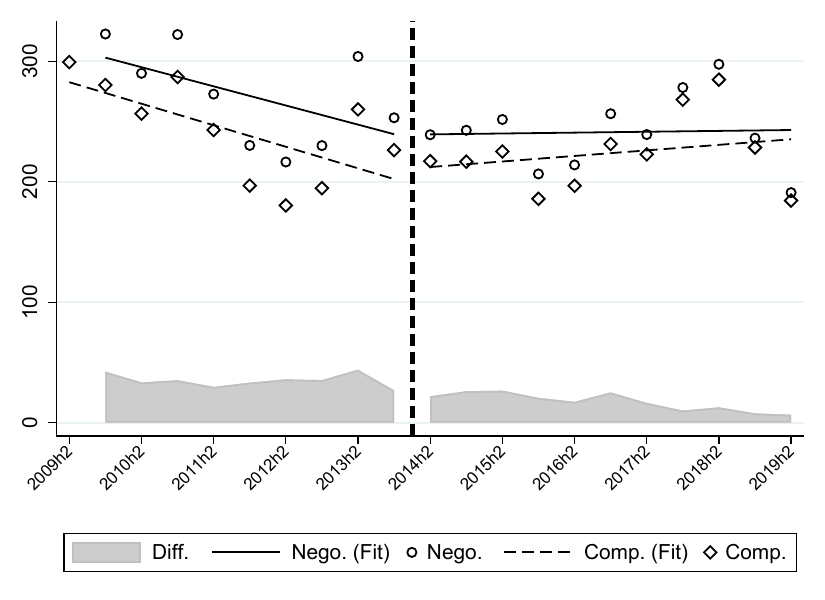}
% \label{fig:muni_adv_fees}

\caption{\footnotesize{This figure reports the binscatter of offering yields  in basis points on the y-axis. Each dot is the average of the offering yields calculated on every $5^{th}$ percentile of the sample for treated and control bonds, separately. The figure also shows the corresponding fitted lines for the negotiated and competitively bid bonds. The difference between the two groups is represented in the shaded portion. The observed pattern suggests a convergence of yields between the treated and control bonds after the SEC Municipal Advisor Rule. This analysis should be interpreted in a non-causal way, as no fixed effect and controls are included.}}
\label{fig:bin_yields}
\end{figure}

\begin{figure}
    \raggedright\textbf{Offering Yields}\\
    \begin{subfigure}{\linewidth}
    \centering
    \includegraphics[scale=.7]{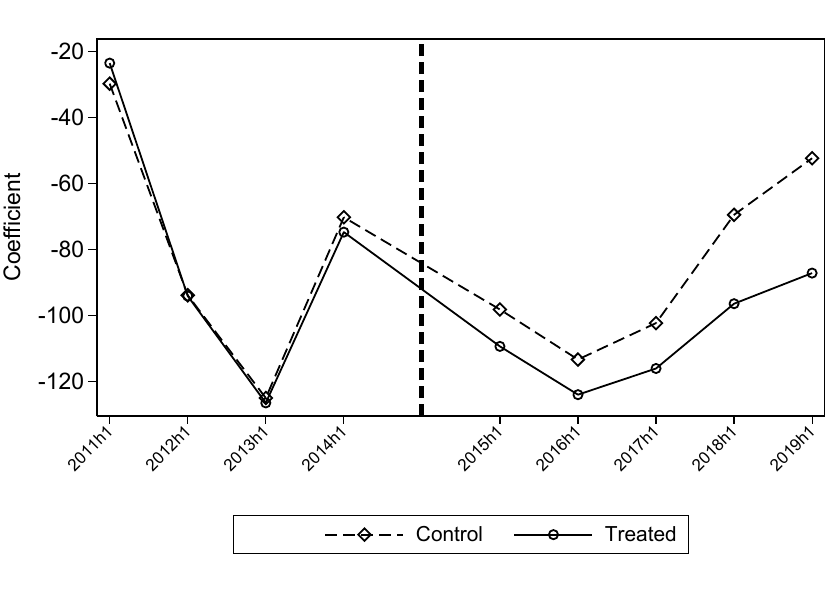}
    
    \caption{} 
    % \label{fig:issuance}
    \end{subfigure}
    
    \medskip
    \raggedright\textbf{Difference in Offering Yields}\\
    \begin{subfigure}{\linewidth}
    \centering
    \includegraphics[scale=.7]{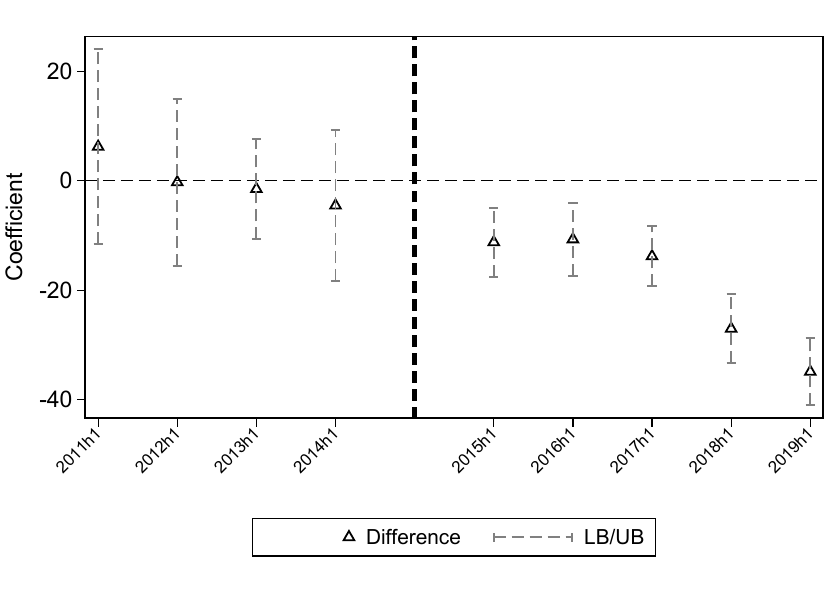}
    \caption{} 
    % \label{fig:issuance_byDebt}
    \end{subfigure}
    
\caption{\textbf{Baseline Result}: \footnotesize{In this figure, I plot the offering yield for new municipal bonds using Equation \eqref{eq:dyn_yield_CompNego} in Panel (a). Panel (b) shows the differences between the yields of treated and control bonds. See Table \ref{table:vardescription} for variables description. The coefficients are shown in basis points. Specifically, I regress the offering yields on yearly interaction dummies for treated and control bonds using issuer fixed effects. These coefficients are depicted on a yearly scale on the x-axis, where the vertical line corresponds to the Municipal Advisor Rule. The omitted benchmark period is the twelve month period before the event window shown above. Standard errors are clustered by state. The dashed lines represent 95\% confidence intervals.}}
\label{fig:did_yield}
\end{figure}

\begin{figure}
    \raggedright\textbf{Issue Yields}\\
    \begin{subfigure}{\linewidth}
    \centering
    \includegraphics[scale=.7]{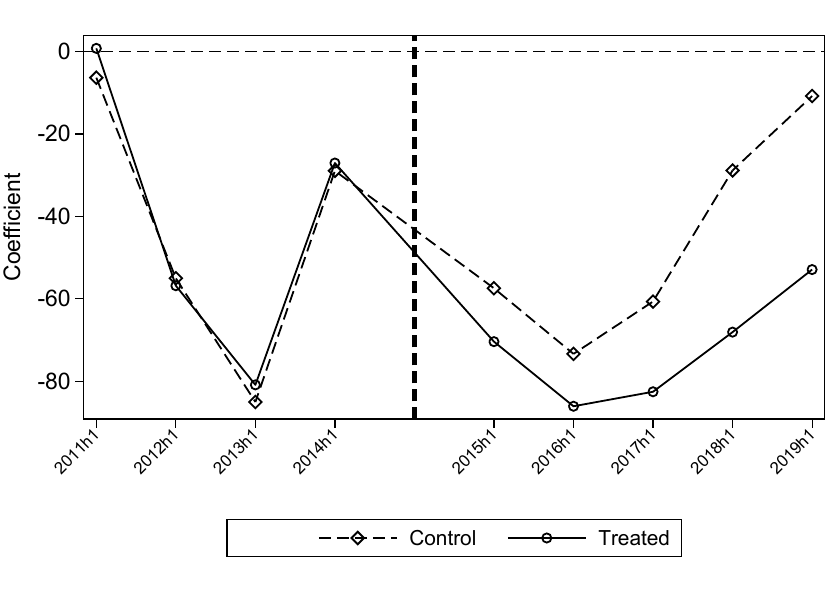}
    
    \caption{} 
    % \label{fig:issuance}
    \end{subfigure}
    
    \medskip
    \raggedright\textbf{Difference in Issue Yields}\\
    \begin{subfigure}{\linewidth}
    \centering
    \includegraphics[scale=.7]{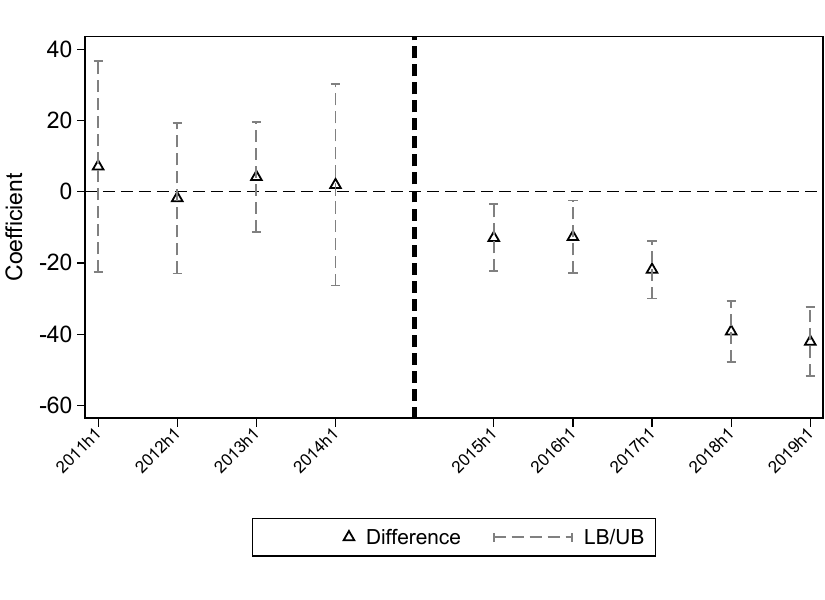}
    \caption{} 
    % \label{fig:issuance_byDebt}
    \end{subfigure}
    
\caption{\textbf{Baseline Result}: \footnotesize{In this figure, I plot the average offering yield for new municipal bond issues using Equation \eqref{eq:dyn_yield_CompNego} in Panel (a). Panel (b) shows the differences between the yields of treated and control bonds. See Table \ref{table:vardescription} for variables description. The coefficients are shown in basis points. Specifically, I regress the average issue yields on yearly interaction dummies for treated and control bonds using issuer fixed effects. These coefficients are depicted on a yearly scale on the x-axis, where the vertical line corresponds to the Municipal Advisor Rule. The omitted benchmark period is the twelve month period before the event window shown above. Standard errors are clustered by state. The dashed lines represent 95\% confidence intervals.}}
\label{fig:did_issuYield}
\end{figure}

\begin{figure}
    \raggedright\textbf{Yield Spreads (Refunding Bonds)}\\
    \begin{subfigure}{\linewidth}
    \centering
    \includegraphics[scale=0.7]{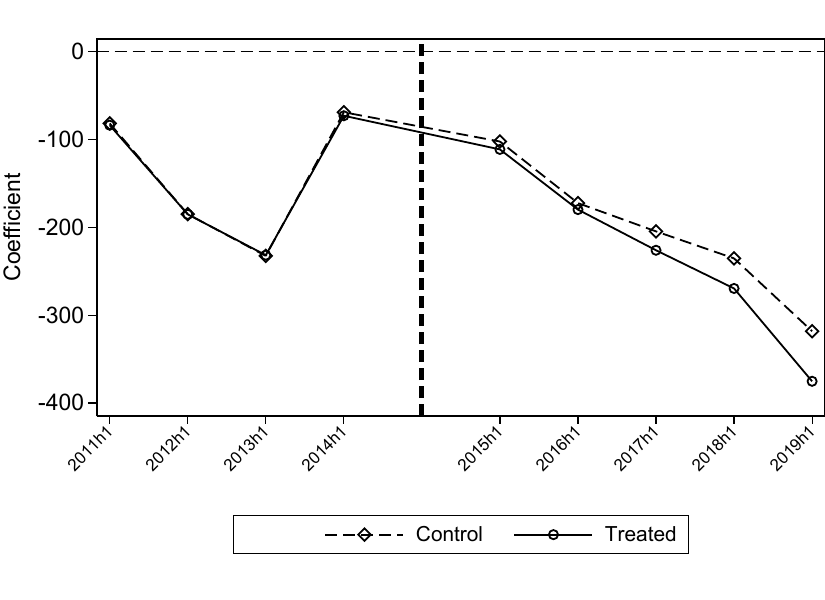}
    \caption{} 
    % \label{fig:issuance}
    \end{subfigure}
    
    \medskip
    \raggedright\textbf{Difference in Yield Spreads (Refunding Bonds)}\\
    \begin{subfigure}{\linewidth}
    \centering
    \includegraphics[scale=0.7]{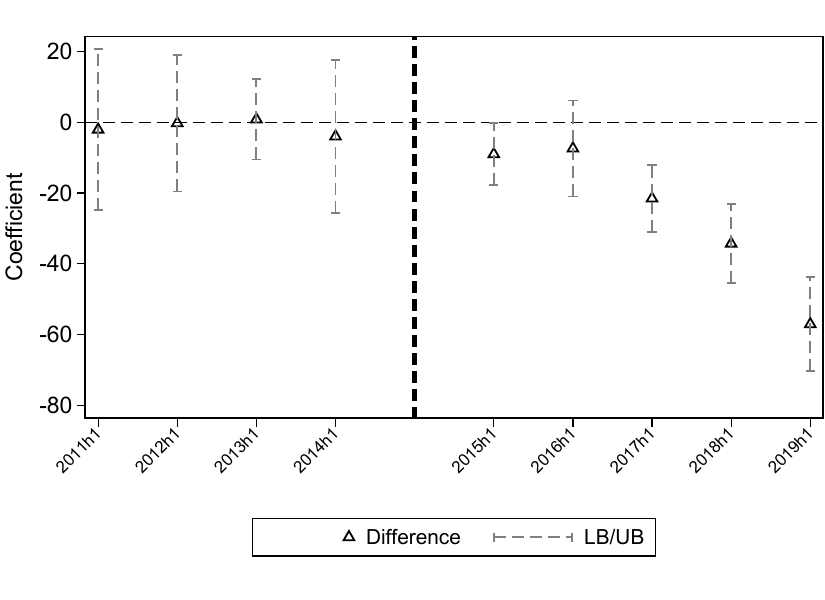}
    \caption{} 
    % \label{fig:issuance_byDebt}
    \end{subfigure}
    
\caption{\textbf{Refunding Bonds}: \footnotesize{In this figure, I plot the average yield spread for refunding municipal bonds issued based on Equation \eqref{eq:dyn_yield_CompNego} in Panel (a). Panel (b) shows the differences between the spreads of treated and control bonds. See Table \ref{table:vardescription} for variables description. The coefficients are shown in basis points. Specifically, the coefficients are obtained from regressing the spreads on yearly interaction dummies for treated and control bonds using issuer fixed effects. These coefficients are depicted on a yearly scale on the x-axis, where the vertical line corresponds to the Municipal Advisor Rule. The omitted benchmark period is the twelve month period before the event window shown above. Standard errors are clustered by state. The dashed lines represent 95\% confidence intervals.}}
\label{fig:REF_spread}
\end{figure}

\begin{figure}
    \raggedright\textbf{$\Delta$(Calling - Refunding) in days}\\
    \begin{subfigure}{\linewidth}
    \centering
    \includegraphics[scale=.75]{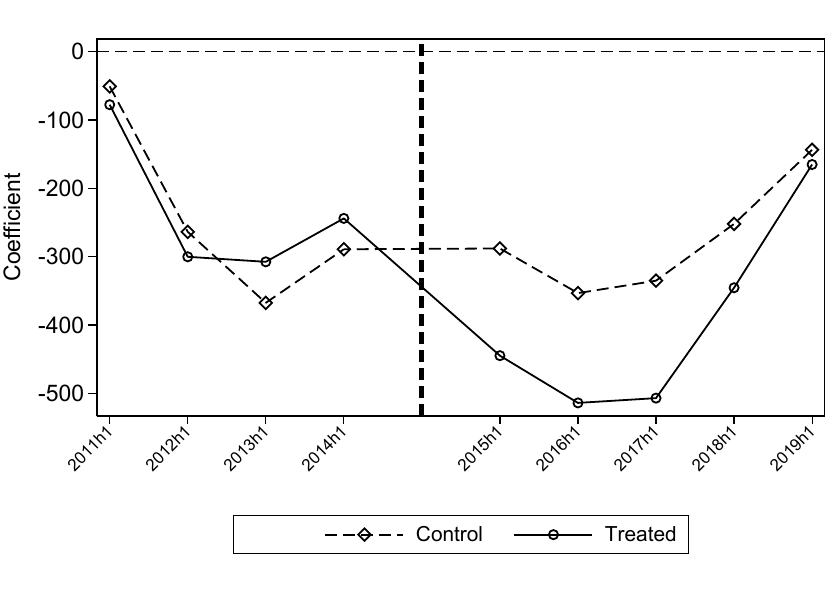}
    
    \caption{} 
    \label{fig:timing_ref_coeff}
    \end{subfigure}
    
    \medskip
    \raggedright\textbf{Difference in $\Delta$(Calling - Refunding) in days}\\
    \begin{subfigure}{\linewidth}
    \centering
    \includegraphics[scale=.75]{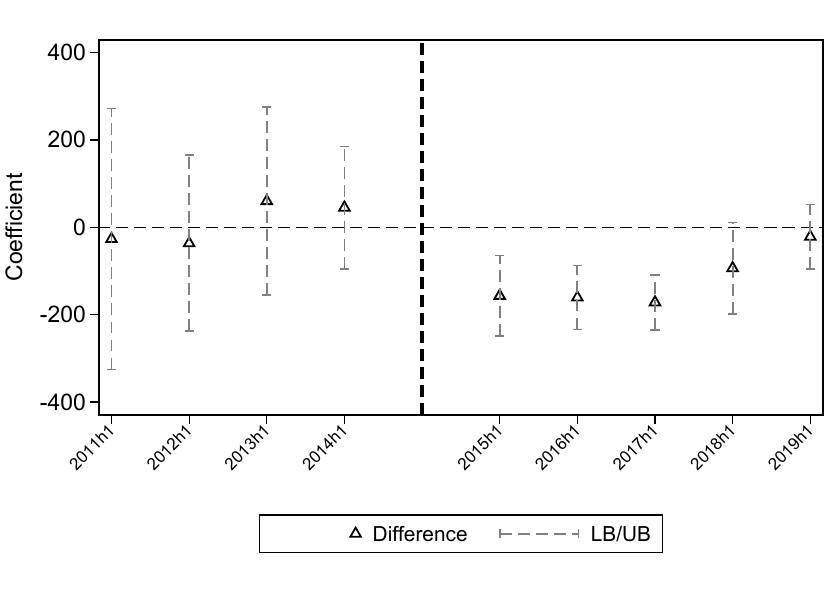}
    \caption{} 
    \label{fig:timing_ref_diff}
    \end{subfigure}
    
\caption{\textbf{Timing of Pre-Refunding Bonds}: \footnotesize{In this figure, I plot the average gap between calling and refunding dates (in days) for pre-refunding municipal bonds using Equation \eqref{eq:dyn_yield_CompNego} in Panel (a). Panel (b) shows the differences between the gap for treated and control bonds. See Table \ref{table:vardescription} for variables description. The coefficients are shown in number of days. Specifically, I regress the gap between calling and refunding days on yearly interaction dummies for treated and control bonds using issuer fixed effects. I depict these coefficients on a yearly scale on the x-axis, where the thick vertical line corresponds to the effective date of the Municipal Advisor Rule. The omitted benchmark period is the twelve month period before the event window shown above. Standard errors are clustered by state. The dashed lines represent 95\% confidence intervals.}}
\label{fig:timing_refunding_typeL}
\end{figure}

% \begin{figure}
% \begin{center}
% \textbf{Refunding vs Refunded bonds}
% \end{center}
% \centering
% \includegraphics[scale=1.2]{Figures/advanceRefunding_advBonds.pdf}
% % \label{fig:muni_adv_fees}

% \caption{\footnotesize{This figure plots the monthly time series of the total par amount of municipal bonds refunded, as well as the refunding volume. Par amounts are
% expressed in billions of dollars.}}
% \label{fig:par_refund}
% \end{figure}

% \clearpage

\newpage
\clearpage
\begin{table}[htbp]
\def\sym#1{\ifmmode^{#1}\else\(^{#1}\)\fi}
\caption{Probability of Choosing Negotiated Sale Conditional on Ex-ante Observables}
%See table: Table10__calling_typeL_CCtrl_diff_refIssue_w1
\label{table:like_nego}
\vspace{0.2in}
\par
{\footnotesize This table shows the estimates from a linear probability regression of choice of negotiated sale on issue characteristics. See Section \ref{subsec:selecting_nego} for details. T-statistics are reported in brackets and standard errors are clustered at the state level. \sym{*} \(p<0.10\), \sym{**} \(p<0.05\), \sym{***} \(p<0.01\)}\\
% \vspace{.2in}
\vspace{.05in} 
% \resizebox{0.9\textwidth}{!} {

% \raggedright\textbf{Panel A: Primary Market}\\
\vspace{0.1in}
\centering
\resizebox{0.7\textwidth}{!} {
\begin{tabular}{@{\extracolsep{4pt}}l*{6}{c}}
\hline
                    \emph{Dependent Variable}:&\multicolumn{6}{c}{Likelihood of Negotiation}\\
                    \cline{2-7}\\ &\multicolumn{1}{c}{(1)}&\multicolumn{1}{c}{(2)}&\multicolumn{1}{c}{(3)}&\multicolumn{1}{c}{(4)}&\multicolumn{1}{c}{(5)}&\multicolumn{1}{c}{(6)}\\
\hline
ln(Issue Size)      &       -0.07         &       -0.06         &       -0.14         &       -0.13         &        0.02         &        0.01         \\
                    &     [-0.55]         &     [-0.50]         &     [-1.00]         &     [-0.97]         &      [0.19]         &      [0.17]         \\
[1em]
ln(avg. bond size)  &        0.13         &        0.12         &        0.17         &        0.17         &        0.01         &        0.02         \\
                    &      [0.92]         &      [0.84]         &      [1.18]         &      [1.13]         &      [0.16]         &      [0.18]         \\
[1em]
Coupon              &        0.05\sym{**} &        0.04\sym{**} &        0.03\sym{**} &        0.03\sym{**} &        0.01         &        0.01         \\
                    &      [2.34]         &      [2.34]         &      [2.04]         &      [2.03]         &      [1.11]         &      [1.11]         \\
[1em]
Maturity            &        0.03         &        0.03         &        0.02         &        0.02         &       -0.02         &       -0.02         \\
                    &      [1.44]         &      [1.29]         &      [1.24]         &      [1.10]         &     [-1.18]         &     [-1.17]         \\
[1em]
Callable            &       -0.06\sym{*}  &       -0.06\sym{**} &       -0.02         &       -0.02         &       -0.02         &       -0.02         \\
                    &     [-1.98]         &     [-2.01]         &     [-0.71]         &     [-0.76]         &     [-0.86]         &     [-0.87]         \\
[1em]
Credit Enh.         &       -0.14\sym{*}  &       -0.14\sym{*}  &       -0.04         &       -0.04         &       -0.00         &       -0.00         \\
                    &     [-1.71]         &     [-1.68]         &     [-0.76]         &     [-0.75]         &     [-0.02]         &     [-0.01]         \\
[1em]
Insured             &        0.10\sym{***}&        0.12\sym{***}&        0.07\sym{**} &        0.08\sym{**} &        0.04         &        0.04         \\
                    &      [2.88]         &      [3.26]         &      [2.35]         &      [2.62]         &      [0.88]         &      [0.89]         \\
[1em]
Bank Qualified      &       -0.10\sym{***}&       -0.09\sym{***}&       -0.05\sym{**} &       -0.04\sym{*}  &        0.01         &        0.01         \\
                    &     [-3.42]         &     [-3.19]         &     [-2.10]         &     [-1.80]         &      [0.92]         &      [1.03]         \\
[1em]
Num. of Bonds       &        0.02         &        0.01         &        0.05         &        0.05         &       -0.00         &       -0.00         \\
                    &      [0.19]         &      [0.17]         &      [0.62]         &      [0.60]         &     [-0.03]         &     [-0.00]         \\
[1em]
GO bond             &                     &       -0.08\sym{**} &                     &       -0.08\sym{**} &                     &       -0.03         \\
                    &                     &     [-2.31]         &                     &     [-2.29]         &                     &     [-0.97]         \\
[1em]
Num. of Txns.       &       -0.04\sym{***}&       -0.04\sym{***}&       -0.03\sym{**} &       -0.03\sym{**} &                     &                     \\
                    &     [-3.09]         &     [-2.78]         &     [-2.39]         &     [-2.25]         &                     &                     \\
[1em]
City(Issuer)        &        0.01         &        0.01         &        0.04         &        0.04         &                     &                     \\
                    &      [0.17]         &      [0.16]         &      [0.95]         &      [0.83]         &                     &                     \\
[1em]
County(Issuer)      &        0.05         &        0.05         &        0.08\sym{**} &        0.09\sym{**} &                     &                     \\
                    &      [1.09]         &      [1.14]         &      [2.08]         &      [2.25]         &                     &                     \\
[1em]
State(Issuer)       &        0.20\sym{***}&        0.18\sym{***}&        0.18\sym{***}&        0.16\sym{***}&                     &                     \\
                    &      [4.26]         &      [3.57]         &      [4.58]         &      [3.90]         &                     &                     \\
[1em]
% Constant            &        0.34\sym{**} &        0.39\sym{**} &        0.19         &        0.24         &        0.33\sym{***}&        0.34\sym{***}\\
%                     &      [2.13]         &      [2.39]         &      [1.20]         &      [1.52]         &      [3.80]         &      [4.47]         \\
\hline
Year FE             &$\checkmark$         &$\checkmark$         &$\checkmark$         &$\checkmark$         &$\checkmark$         &$\checkmark$         \\
Purpose FE          &$\checkmark$         &$\checkmark$         &$\checkmark$         &$\checkmark$         &$\checkmark$         &$\checkmark$         \\
Rating FE           &$\checkmark$         &$\checkmark$         &$\checkmark$         &$\checkmark$         &$\checkmark$         &$\checkmark$         \\
State FE            &                     &                     &$\checkmark$         &$\checkmark$         &                     &                     \\
Issuer FE           &                     &                     &                     &                     &$\checkmark$         &$\checkmark$         \\
Adj.-R$^2$          &       0.174         &       0.178         &       0.307         &       0.311         &       0.686         &       0.686         \\
Obs.                &      15,578         &      15,578         &      15,578         &      15,578         &      15,578         &      15,578         \\
\hline
\end{tabular}
}
\end{table}

\begin{table}[htbp]
% \scriptsize
\def\sym#1{\ifmmode^{#1}\else\(^{#1}\)\fi}
\caption{Summary Statistics: Municipal Bonds}
\label{table:summary_bonds}
\vspace{0.2in}
\par
\footnotesize{This table summarizes the municipal bond level characteristics during 2010-2019 for the bonds in the sample. The two panels correspond to the treated (negotiated sale) versus control (competitively bid) bonds. The key variables are described in Table \ref{table:vardescription}.}\vspace{.2in} \\

%  \vspace{.05in}
% \raggedright\textbf{Panel A: Secondary market }\\
\centering
% \textbf{Panel A: Secondary market }\\
\vspace{0.1in}
% \resizebox{0.9\textwidth}{!} {

\begin{tabular}{l*{1}{cccccc}}
\hline
                    &\multicolumn{6}{c}{}                               \\
                    &       Count&        Mean&       Std. Dev.&   P25&  P50& P75         \\
\hline
% \textbf{All Bonds}               &            &            &            &            &            &            \\
% % Issue Size (USD million)&     837,084&       47.71&      128.09&         4.8&        10.4&        35.7\\
% Amount (USD million)&     837,084&        2.71&       10.95&         0.3&         0.6&         1.8\\
% Coupon(\%)          &     837,084&        3.51&        1.13&         2.8&         3.4&         4.7\\
% Years to Maturity   &     837,084&        9.86&        6.16&         5.0&         8.9&        13.9\\
% Offering Price (USD)&     837,083&      106.60&        7.67&       100.0&       103.9&       111.7\\
% Offering Yield(\%)  &     837,084&        2.33&        1.01&         1.5&         2.3&         3.0\\
% Callable            &     837,084&        0.47&        0.50&         0.0&         0.0&         1.0\\
% General Obligation (Dummy)&     837,084&        0.60&        0.49&         0.0&         1.0&         1.0\\
% Bank Qualified (Dummy)&     837,084&        0.40&        0.49&         0.0&         0.0&         1.0\\
% Cred. Enh. (Dummy)  &     837,084&        0.21&        0.41&         0.0&         0.0&         0.0\\
% Insured (Dummy)     &     837,084&        0.16&        0.37&         0.0&         0.0&         0.0\\
% \hline
\textbf{Treated - Negotiated Sale}              &            &            &            &            \\
% \hline
% Issue Size (USD million)&     270,504&       71.59&      165.60&         7.8&        21.5&        64.2\\
Amount (USD million)&     270,504&        4.08&       14.83&         0.4&         1.0&         2.8\\
Coupon(\%)          &     270,504&        3.90&        1.10&         3.0&         4.0&         5.0\\
Years to Maturity   &     270,504&       10.34&        6.50&         5.2&         9.2&        14.4\\
Offering Price (USD)&     270,504&      108.62&        8.30&       101.1&       107.4&       115.1\\
Offering Yield(\%)  &     270,504&        2.47&        1.04&         1.7&         2.4&         3.2\\
Yield Spread(\%)    &     270,504&        1.32&        1.31&         0.4&         1.3&         2.2\\
Callable (Dummy)        &     270,504&        0.47&        0.50&         0.0&         0.0&         1.0\\
General Obligation (Dummy)&     270,504&        0.42&        0.49&         0.0&         0.0&         1.0\\
Bank Qualified (Dummy)&     270,504&        0.23&        0.42&         0.0&         0.0&         0.0\\
Cred. Enh. (Dummy)  &     270,504&        0.13&        0.34&         0.0&         0.0&         0.0\\
Insured (Dummy)     &     270,504&        0.19&        0.40&         0.0&         0.0&         0.0\\
% Markup (bps)        &     250,793&       25.65&       75.70&        -0.0&         0.0&        23.8\\
% Price dispersion (per USD 100)&     250,793&        0.11&        0.20&         0.0&         0.0&         0.1\\
\hline\\
\textbf{Control - Competitively Bid}              &            &            &            &            \\
% Issue Size (USD million)&     564,420&       36.42&      103.82&         3.9&         8.9&        24.7\\
Amount (USD million)&     564,420&        2.04&        8.29&         0.2&         0.5&         1.3\\
Coupon(\%)          &     564,420&        3.33&        1.10&         2.5&         3.0&         4.0\\
Years to Maturity   &     564,420&        9.65&        5.96&         4.9&         8.7&        13.7\\
Offering Price (USD)&     564,419&      105.65&        7.16&       100.0&       103.1&       109.2\\
Offering Yield(\%)  &     564,420&        2.27&        0.99&         1.5&         2.3&         3.0\\
Yield Spread(\%)    &     564,420&        1.27&        1.14&         0.5&         1.2&         2.0\\
Callable (Dummy)&     564,420&        0.47&        0.50&         0.0&         0.0&         1.0\\
General Obligation (Dummy)&     564,420&        0.68&        0.47&         0.0&         1.0&         1.0\\
Bank Qualified (Dummy)&     564,420&        0.48&        0.50&         0.0&         0.0&         1.0\\
Cred. Enh. (Dummy)  &     564,420&        0.24&        0.43&         0.0&         0.0&         0.0\\
Insured (Dummy)     &     564,420&        0.15&        0.35&         0.0&         0.0&         0.0\\
% Markup (bps)        &     535,735&       12.55&       75.74&        -0.1&         0.0&        16.0\\
% Price dispersion (per USD 100)&     535,735&        0.13&        0.22&         0.0&         0.0&         0.2\\
\hline
\end{tabular}
% }
\end{table}

\clearpage
\newpage
\begin{table}[htbp]
% \centering
\def\sym#1{\ifmmode^{#1}\else\(^{#1}\)\fi}
% \scriptsize
\caption{Robustness Tests}
\label{table:robustness}
\vspace{0.2in}
\par
{\footnotesize In this table I report results for various robustness tests on the baseline specification, i.e., Column (8) of Table \ref{table:main_baseline}. Columns (1)-(2) show the baseline effect by changing the dependent variable to after-tax yield and after-tax yield spread, respectively. In Columns (3)-(11), I report results based on alternative econometric specifications. I introduce additional fixed effects to account for unobserved factors that may be varying over time. Specifically, Column (3) reports baseline results by adding issuer-type $\times$ year fixed effects. Column (4) shows results by adding bond purpose fixed effects. I add bond purpose $\times$ year fixed effect in Column (5). Columns (6) and (7) show results by adding underwriter fixed effect and underwriter $\times$ year fixed effect, respectively. In Columns (8) and (9), I control for unobserved pairing between issuers and advisors, as well as issuers and underwriters, separately, by adding issuer-advisor pair fixed effect and issuer-underwriter pair fixed effect, respectively. These specifications include time unvarying advisor and underwriter fixed effects, respectively. Column (10) shows results with advisor $\times$ state fixed effects. In Column (11), I also add county $\times$ year fixed effects. I consider additional tax considerations in Columns (12)-(14). First, I relax the sample of bonds to include taxable bonds in Columns (12)-(13). In Column (13), I further omit bonds from five states (IL, IA, KS, OK, WI) that tax interest income on municipal bonds issued in-state or out-of-state \citep{gao2021good}. Column (14) shows results using bonds that are exempt from both state and federal income tax simultaneously. Columns (15)-(18) report results focusing on sub-samples of homogeneous bonds. Accordingly, in Column (15), I drop bonds in which the advisor and underwriter are same. Column (16) shows results by dropping callable bonds. I drop insured bonds in Column (17). Finally, I focus on only the new money bonds in Column (18). The results in Columns (19)-(21) focus on additional geographic considerations. I keep only local bonds (by dropping state level bonds) in Column (19). Conversely, I show results using only the state level bonds in Column (20). In Column (21), I report the baseline results by dropping issuances from the three largest municipal bond issuers, namely: California (CA), New York (NY) and Texas (TX). I consider alternative levels of clustering standard errors in Columns (22)-(32). In Columns (22)-(26), I cluster standard errors by advisor, underwriter, issuer, issuer(2), and bond issue, respectively. Issuer(2) in Column (25) refers to weakly identifying borrowers based on the first six-digits of the bond CUSIP \citep{gao2021good}. Columns (27)-(28) double cluster standard errors along two dimensions in the geography of issuers: state-advisor, and advisor-issuer, respectively. Finally, in Columns (29)-(32), I double cluster standard errors over time and across bonds using: state and year, advisor and year, state and year-month, and advisor and year-month, respectively. In Table \ref{table:robustness_yld}, I replicate these results using offering yield as the dependent variable. Additionally, I report robustness results for offering price as the dependent variable in Table \ref{table:robustness_offPrice}. T-statistics are reported in brackets and standard errors are clustered at the state level, unless otherwise specified. \sym{*} \(p<0.10\), \sym{**} \(p<0.05\), \sym{***} \(p<0.01\)}\\
\end{table}
\clearpage
\newpage
\begin{landscape}
\begin{table}
    \centering
    \def\sym#1{\ifmmode^{#1}\else\(^{#1}\)\fi}
    \vspace{0.2cm}
    \resizebox{1.3\textwidth}{!}{
\begin{tabular}{@{\extracolsep{4pt}}l*{11}{c}@{}}
\hline
                    \emph{Dependent Variable}: &\multicolumn{11}{c}{ Yield Spread (basis points)} \vspace{0.2in} \\
                    &\multicolumn{2}{c}{Other Dependent Variables}&\multicolumn{9}{c}{Alternative Specifications}\\
                    \cline{2-3} \cline{4-12}  \\
                    &\multicolumn{1}{c}{After-tax  }&\multicolumn{1}{c}{After-tax }&\multicolumn{1}{c}{Add Issuer-Type}&\multicolumn{1}{c}{Add}&\multicolumn{1}{c}{Add Purpose}&\multicolumn{1}{c}{Add }&\multicolumn{1}{c}{Add }&\multicolumn{1}{c}{Add }&\multicolumn{1}{c}{Add}&\multicolumn{1}{c}{Add}&\multicolumn{1}{c}{Add}\\                   &\multicolumn{1}{c}{Yield}&\multicolumn{1}{c}{Yield Spread}&\multicolumn{1}{c}{Year FE}&\multicolumn{1}{c}{Purpose FE}&\multicolumn{1}{c}{Year FE}&\multicolumn{1}{c}{UW FE}&\multicolumn{1}{c}{UW-Yr. FE}&\multicolumn{1}{c}{Iss.-MA FE}&\multicolumn{1}{c}{Iss.-UW FE}&\multicolumn{1}{c}{MA-State FE}&\multicolumn{1}{c}{County-Yr. FE}\\ &\multicolumn{1}{c}{(1)}&\multicolumn{1}{c}{(2)}&\multicolumn{1}{c}{(3)}&\multicolumn{1}{c}{(4)}&\multicolumn{1}{c}{(5)}&\multicolumn{1}{c}{(6)}&\multicolumn{1}{c}{(7)}&\multicolumn{1}{c}{(8)}&\multicolumn{1}{c}{(9)}&\multicolumn{1}{c}{(10)}&\multicolumn{1}{c}{(11)}\\
\hline\\
\vspace{0.2cm}
Treated $\times$ Post &      -18.13\sym{***}&      -19.69\sym{***}&      -12.02\sym{***}&      -12.63\sym{***}&      -12.19\sym{***}&      -12.92\sym{***}&      -11.07\sym{***}&      -14.13\sym{***}&      -14.20\sym{**} &      -11.88\sym{***}&      -10.65\sym{***}\\
                    &     [-4.23]         &     [-4.33]         &     [-4.05]         &     [-4.19]         &     [-3.86]         &     [-4.45]         &     [-3.49]         &     [-4.25]         &     [-2.60]         &     [-3.86]         &     [-3.01]         \\
[1em]
Adj.-R$^2$          &       0.867         &       0.853         &       0.855         &       0.855         &       0.855         &       0.856         &       0.860         &       0.857         &       0.891         &       0.856         &       0.871         \\
Obs.                &     833,343         &     833,343         &     833,667         &     833,348         &     833,348         &     834,730         &     834,707         &     834,670         &     834,297         &     834,731         &     834,629         \\
\hline
\end{tabular}
}\\

% \vspace{1cm}
\medskip
% \vspace{-2em}
   \resizebox{1.3\textwidth}{!}{
\begin{tabular}{@{\extracolsep{4pt}}l*{10}{c}@{}}

                    \emph{Dependent Variable}: &\multicolumn{10}{c}{ Yield Spread (basis points)} \vspace{0.2in}\\
                    \cline{2-11} \\
                    &\multicolumn{3}{c}{Tax Considerations}&\multicolumn{4}{c}{Bond Considerations}&\multicolumn{3}{c}{Geographic Considerations}\\
                    \cline{2-4}  \cline{5-8} \cline{9-11} \\ &\multicolumn{2}{c}{Include Taxable}&\multicolumn{1}{c}{Exempt}&\multicolumn{1}{c}{Drop same}&\multicolumn{1}{c}{Drop}&\multicolumn{1}{c}{Drop}&\multicolumn{1}{c}{Only}&\multicolumn{1}{c}{Keep}&\multicolumn{1}{c}{Keep}&\multicolumn{1}{c}{Drop}\\     \cline{2-3}\vspace{-1em}\\  &\multicolumn{1}{c}{}&\multicolumn{1}{c}{(-Taxable States)}&\multicolumn{1}{c}{(Fed.+State)}&\multicolumn{1}{c}{Adv.-UW. bonds}&\multicolumn{1}{c}{Callable}&\multicolumn{1}{c}{Insured}&\multicolumn{1}{c}{New money}&\multicolumn{1}{c}{Local}&\multicolumn{1}{c}{State}&\multicolumn{1}{c}{CA,NY,TX}\\                    &\multicolumn{1}{c}{(12)}&\multicolumn{1}{c}{(13)}&\multicolumn{1}{c}{(14)}&\multicolumn{1}{c}{(15)}&\multicolumn{1}{c}{(16)}&\multicolumn{1}{c}{(17)}&\multicolumn{1}{c}{(18)}&\multicolumn{1}{c}{(19)}&\multicolumn{1}{c}{(20)}&\multicolumn{1}{c}{(21)}\\
\hline\\
\vspace{0.2cm}
Treated $\times$ Post &      -11.93\sym{***}&      -11.08\sym{***}&      -11.94\sym{***}&      -12.64\sym{***}&      -11.44\sym{***}&      -14.88\sym{***}&      -22.90\sym{***}&      -10.81\sym{***}&      -17.15\sym{**} &      -15.94\sym{***}\\
                    &     [-4.39]         &     [-4.23]         &     [-4.07]         &     [-4.32]         &     [-5.53]         &     [-5.92]         &     [-4.96]         &     [-3.50]         &     [-2.59]         &     [-5.77]         \\
[1em]
Adj.-R$^2$          &       0.836         &       0.834         &       0.854         &       0.854         &       0.876         &       0.856         &       0.880         &       0.861         &       0.836         &       0.859         \\
Obs.                &     905,084         &     794,062         &     770,446         &     830,458         &     443,572         &     698,776         &     415,926         &     751,278         &      83,456         &     519,544         \\
\hline
\end{tabular}
}\\

% \vspace{1cm}
% \vspace{-2em}
\medskip
   \resizebox{1.3\textwidth}{!}{
\begin{tabular}{@{\extracolsep{4pt}}l*{11}{c}@{}}
                    \emph{Dependent Variable}: &\multicolumn{11}{c}{ Yield Spread (basis points)} \vspace{0.2in} \\
                    \cline{2-12} \\
                    &\multicolumn{11}{c}{Alternative Clustering}\\
                    \cline{2-12}\\                    &\multicolumn{1}{c}{Advisor}&\multicolumn{1}{c}{Underwriter}&\multicolumn{1}{c}{Issuer}&\multicolumn{1}{c}{Issuer(2)}&\multicolumn{1}{c}{Issue}&\multicolumn{1}{c}{State, Advisor}&\multicolumn{1}{c}{Advisor, Issuer}&\multicolumn{1}{c}{State, Year}&\multicolumn{1}{c}{Advisor, Year}&\multicolumn{1}{c}{State, YM}&\multicolumn{1}{c}{Advisor, YM}\\    &\multicolumn{1}{c}{(22)}&\multicolumn{1}{c}{(23)}&\multicolumn{1}{c}{(24)}&\multicolumn{1}{c}{(25)}&\multicolumn{1}{c}{(26)}&\multicolumn{1}{c}{(27)}&\multicolumn{1}{c}{(28)}&\multicolumn{1}{c}{(29)}&\multicolumn{1}{c}{(30)}&\multicolumn{1}{c}{(31)}&\multicolumn{1}{c}{(32)}\\
\hline\\
\vspace{0.2cm}
Treated $\times$ Post &      -12.60\sym{***}&      -12.60\sym{***}&      -12.60\sym{***}&      -12.60\sym{***}&      -12.60\sym{***}&      -12.60\sym{***}&      -12.60\sym{***}&      -12.60\sym{***}&      -12.60\sym{***}&      -12.60\sym{***}&      -12.60\sym{***}\\
                    &     [-4.85]         &     [-6.42]         &     [-6.40]         &     [-8.40]         &     [-9.92]         &     [-3.99]         &     [-4.47]         &     [-3.49]         &     [-3.43]         &     [-4.12]         &     [-4.59]         \\
[1em]
Adj.-R$^2$          &       0.855         &       0.855         &       0.855         &       0.855         &       0.855         &       0.855         &       0.855         &       0.855         &       0.855         &       0.855         &       0.855         \\
Obs.                &     834,741         &     834,741         &     834,741         &     834,741         &     834,741         &     834,741         &     834,741         &     834,741         &     834,741         &     834,741         &     834,741         \\
\hline
\end{tabular}
}
\end{table}
\end{landscape}

\begin{landscape}
\begin{table}[htbp]
\def\sym#1{\ifmmode^{#1}\else\(^{#1}\)\fi}
\caption{Impact on Offering Yields of Local Governments: Evidence from  Municipal Bonds Primary Market} 
\label{table:baseline_yld}
\vspace{0.2in}
\par
{\footnotesize This table reports the baseline results for my sample using Equation \eqref{eq:baseline} estimating the differential effect on municipal bond yields of treated and control bonds after the Municipal Advisor Rule of 2014. The primary coefficient of interest, $\beta_0$, is captured by the interaction term of \textit{Treated $\times$ Post}. I show the results using offering yields as the dependent variable. Specifically, Column (1) reports the results without any controls or fixed effects. In Column (2), I first introduce issuer fixed effects. Column (3) shows results by introducing state $\times$ year fixed effects. In Column (4), I add advisor fixed effect. Column (5) reports the results by additionally including bond level controls consisting of coupon (\%); log(amount issued in \$); dummies for callable bonds, bond insurance, general obligation bond, bank qualification, refunding and credit enhancement; credit rating; remaining years to maturity; and inverse years to maturity. I provide the description of key variables in Table \ref{table:vardescription}. In Column (6), I control for the county-level economic conditions. I use the lagged values for log(labor force) and unemployment rate, and the percentage change in unemployment rate and labor force, respectively. Column (7) replaces advisor fixed effect with advisor $\times$ year fixed effect and does not include county-level controls. Finally, Column (8) shows results by also adding county-level controls. T-statistics are reported in brackets and standard errors are clustered at the state level. \sym{*} \(p<0.10\), \sym{**} \(p<0.05\), \sym{***} \(p<0.01\)}\\
% \vspace{.2in}
\vspace{.05in} 
% \resizebox{0.9\textwidth}{!} {

% \raggedright\textbf{Panel A: Primary Market}\\
\vspace{0.1in}
\centering
\resizebox{1.25\textwidth}{!} {
\begin{tabular}{@{\extracolsep{4pt}}l*{8}{c}}
\hline
                    \emph{Dependent Variable}:&\multicolumn{8}{c}{Offering Yield (basis points)}\\
                    \cline{2-9}\\                    &\multicolumn{1}{c}{(1)}&\multicolumn{1}{c}{(2)}&\multicolumn{1}{c}{(3)}&\multicolumn{1}{c}{(4)}&\multicolumn{1}{c}{(5)}&\multicolumn{1}{c}{(6)}&\multicolumn{1}{c}{(7)}&\multicolumn{1}{c}{(8)}\\
                    % &\multicolumn{3}{c}{Yield}&\multicolumn{3}{c}{Spread}&\multicolumn{3}{c}{yield spread}\\
\hline
Treated $\times$ Post &      -17.62\sym{***}&      -20.84\sym{***}&      -11.10\sym{***}&      -10.60\sym{***}&      -13.96\sym{***}&      -13.92\sym{***}&      -11.10\sym{***}&      -11.08\sym{***}\\
                    &     [-2.78]         &     [-2.72]         &     [-2.75]         &     [-2.75]         &     [-4.79]         &     [-4.78]         &     [-4.14]         &     [-4.14]         \\
[1em]
Treated             &       31.55\sym{***}&       -2.18         &       -1.93         &       -2.80         &        8.98\sym{***}&        8.98\sym{***}&        7.44\sym{**} &        7.45\sym{**} \\
                    &      [2.91]         &     [-0.23]         &     [-0.32]         &     [-0.46]         &      [2.70]         &      [2.71]         &      [2.11]         &      [2.11]         \\
[1em]
Post                &      -11.60\sym{***}&      -14.28\sym{***}&      -10.23\sym{***}&      -11.05\sym{***}&       -8.40\sym{***}&       -8.34\sym{***}&       -9.19\sym{***}&       -9.14\sym{***}\\
                    &     [-3.64]         &     [-2.93]         &     [-4.78]         &     [-5.20]         &     [-4.92]         &     [-4.88]         &     [-5.55]         &     [-5.50]         \\
[1em]
\hline
Issuer FE      &                     &$\checkmark$         &$\checkmark$         &$\checkmark$         &$\checkmark$         &$\checkmark$         &$\checkmark$          &$\checkmark$         \\
State-Year FE       &                     &                     &$\checkmark$         &$\checkmark$         &$\checkmark$         &$\checkmark$         &$\checkmark$         &$\checkmark$         \\
Advisor FE             &                     &                     &                     &$\checkmark$         &$\checkmark$         &$\checkmark$         &          &   \\
Bond Controls     &                     &                     &                     &                     &$\checkmark$         &$\checkmark$         &$\checkmark$         &$\checkmark$         \\
County Controls           &                     &                     &                     &                     &                     &$\checkmark$         &         &$\checkmark$         \\
Advisor-Year FE          &                     &                     &                     &                     &                     &      & $\checkmark$ &$\checkmark$         \\
Adj.-R$^2$          &       0.017         &       0.197         &       0.263         &       0.267         &       0.862         &       0.862         &       0.868         &       0.868         \\
Obs.                &     834,925         &     834,764         &     834,764         &     834,760         &     834,760         &     834,760         &     834,741         &     834,741         \\
\hline
\end{tabular}
}
\end{table}
\end{landscape}
\clearpage

\begin{landscape}
\begin{table}[htbp]
\def\sym#1{\ifmmode^{#1}\else\(^{#1}\)\fi}
\caption{Impact on  Amihud Measure (Liquidity) of New Bonds} 
\label{table:baseline_amihud}
\vspace{0.2in}
\par
{\footnotesize This table reports the baseline results for the sample using Equation \eqref{eq:baseline} estimating the differential effect on Amihud measure of liquidity between treated and control bonds after the Municipal Advisor Rule of 2014. I use trades during the first month after issuance to construct this measure using \cite{schwert2017municipal}, based on \cite{amihud2002}. The primary coefficient of interest, $\beta_0$, is captured by the interaction term of \textit{Treated $\times$ Post}. Specifically, Column (1) reports the results without any controls or fixed effects. In Column (2), I first introduce issuer fixed effects. Column (3) shows results by introducing state $\times$ year fixed effects. In Column (4), I add advisor fixed effect. Column (5) reports the results by additionally including bond level controls consisting of coupon (\%); log(amount issued in \$); dummies for callable bonds, bond insurance, general obligation bond, bank qualification, refunding and credit enhancement; credit rating; remaining years to maturity; and inverse years to maturity. I provide the description of key variables in Table \ref{table:vardescription}. In Column (6), I control for the county-level economic conditions. I use the lagged values for log(labor force) and unemployment rate, and the percentage change in unemployment rate and labor force, respectively. Column (7) replaces advisor fixed effect with advisor $\times$ year fixed effect and does not include county-level controls. Finally, Column (8) shows results by also adding county-level controls. T-statistics are reported in brackets and standard errors are clustered at the state level. \sym{*} \(p<0.10\), \sym{**} \(p<0.05\), \sym{***} \(p<0.01\)}\\
% \vspace{.2in}
\vspace{.05in} 
% \resizebox{0.9\textwidth}{!} {

% \raggedright\textbf{Panel A: Primary Market}\\
\vspace{0.1in}
\centering
\resizebox{1.25\textwidth}{!} {
\begin{tabular}{@{\extracolsep{4pt}}l*{8}{c}}
\hline
                    \emph{Dependent Variable}:&\multicolumn{8}{c}{Amihud measure}\\
                    \cline{2-9}\\                    &\multicolumn{1}{c}{(1)}&\multicolumn{1}{c}{(2)}&\multicolumn{1}{c}{(3)}&\multicolumn{1}{c}{(4)}&\multicolumn{1}{c}{(5)}&\multicolumn{1}{c}{(6)}&\multicolumn{1}{c}{(7)}&\multicolumn{1}{c}{(8)}\\
\hline
Treated $\times$ Post &       -2.53\sym{***}&       -2.19\sym{***}&       -1.67\sym{***}&       -1.58\sym{***}&       -1.67\sym{***}&       -1.66\sym{***}&       -1.47\sym{***}&       -1.46\sym{***}\\
                    &     [-5.68]         &     [-6.37]         &     [-4.82]         &     [-4.67]         &     [-8.37]         &     [-8.30]         &     [-7.65]         &     [-7.62]         \\
[1em]
Treated             &       -1.87\sym{***}&       -2.93\sym{***}&       -3.21\sym{***}&       -3.30\sym{***}&       -1.29\sym{***}&       -1.29\sym{***}&       -1.40\sym{***}&       -1.40\sym{***}\\
                    &     [-4.69]         &     [-8.83]         &     [-9.23]         &     [-9.34]         &     [-7.18]         &     [-7.20]         &     [-8.04]         &     [-8.07]         \\
[1em]
Post                &        2.41\sym{***}&        1.86\sym{***}&        0.47         &        0.43         &        0.72\sym{***}&        0.72\sym{***}&        0.56\sym{**} &        0.56\sym{**} \\
                    &      [8.21]         &      [5.72]         &      [1.54]         &      [1.44]         &      [2.75]         &      [2.76]         &      [2.03]         &      [2.02]         \\
[1em]
\hline
Issuer FE      &                     &$\checkmark$         &$\checkmark$         &$\checkmark$         &$\checkmark$         &$\checkmark$         &$\checkmark$          &$\checkmark$         \\
State-Year FE       &                     &                     &$\checkmark$         &$\checkmark$         &$\checkmark$         &$\checkmark$         &$\checkmark$         &$\checkmark$         \\
Advisor FE             &                     &                     &                     &$\checkmark$         &$\checkmark$         &$\checkmark$         &          &   \\
Bond Controls     &                     &                     &                     &                     &$\checkmark$         &$\checkmark$         &$\checkmark$         &$\checkmark$         \\
County Controls           &                     &                     &                     &                     &                     &$\checkmark$         &         &$\checkmark$         \\
Advisor-Year FE          &                     &                     &                     &                     &                     &      & $\checkmark$ &$\checkmark$         \\
Adj.-R$^2$          &       0.014         &       0.107         &       0.112         &       0.113         &       0.277         &       0.277         &       0.281         &       0.281         \\
Obs.                &     526,910         &     526,285         &     526,285         &     526,278         &     526,278         &     526,278         &     526,245         &     526,245         \\
\hline
\end{tabular}
}
\end{table}
\end{landscape}

\begin{landscape}
\begin{table}[htbp]
\def\sym#1{\ifmmode^{#1}\else\(^{#1}\)\fi}
\caption{Impact on Offering Yields of Local Governments using Issue Yields} 
\label{table:issu_yld}
\vspace{0.2in}
\par
{\footnotesize This table reports the baseline results for the sample using Equation \eqref{eq:baseline} estimating the differential effect on municipal issue yields of treated and control bonds at the issue level, after the Municipal Advisor Rule of 2014. The primary coefficient of interest, $\beta_0$, is captured by the interaction term of \textit{Treated $\times$ Post}. Specifically, Column (1) reports the results without any controls or fixed effects. In Column (2), I first introduce issuer fixed effects. Column (3) shows results by introducing state $\times$ year fixed effects. In Column (4), I add advisor fixed effect. Column (5) reports the results by additionally including bond level controls consisting of coupon (\%); log(amount issued in \$); dummies for callable bonds, bond insurance, general obligation bond, bank qualification, refunding and credit enhancement; credit rating; remaining years to maturity; and inverse years to maturity. I provide the description of key variables in Table \ref{table:vardescription}. In Column (6), I control for the county-level economic conditions. I use the lagged values for log(labor force) and unemployment rate, and the percentage change in unemployment rate and labor force, respectively. Column (7) replaces advisor fixed effect with advisor $\times$ year fixed effect and does not include county-level controls. Finally, Column (8) shows results by also adding county-level controls. T-statistics are reported in brackets and standard errors are clustered at the state level. \sym{*} \(p<0.10\), \sym{**} \(p<0.05\), \sym{***} \(p<0.01\)}\\
% \vspace{.2in}
\vspace{.05in} 
% \resizebox{0.9\textwidth}{!} {

% \raggedright\textbf{Panel A: Primary Market}\\
\vspace{0.1in}
\centering
\resizebox{1.25\textwidth}{!} {
\begin{tabular}{@{\extracolsep{4pt}}l*{8}{c}}
\hline
                    \emph{Dependent Variable}:&\multicolumn{8}{c}{Issue Level Offering Yield (basis points)}\\
                    \cline{2-9}\\                    &\multicolumn{1}{c}{(1)}&\multicolumn{1}{c}{(2)}&\multicolumn{1}{c}{(3)}&\multicolumn{1}{c}{(4)}&\multicolumn{1}{c}{(5)}&\multicolumn{1}{c}{(6)}&\multicolumn{1}{c}{(7)}&\multicolumn{1}{c}{(8)}\\
                    % &\multicolumn{3}{c}{Yield}&\multicolumn{3}{c}{Spread}&\multicolumn{3}{c}{yield spread}\\
\hline
Treated $\times$ Post &      -27.38\sym{***}&      -29.74\sym{***}&      -15.67\sym{**} &      -14.50\sym{**} &      -17.60\sym{***}&      -17.55\sym{***}&      -14.10\sym{***}&      -14.08\sym{***}\\
                    &     [-3.30]         &     [-2.92]         &     [-2.28]         &     [-2.20]         &     [-4.34]         &     [-4.34]         &     [-3.78]         &     [-3.78]         \\
[1em]
Treated             &       53.90\sym{***}&        1.97         &       -0.54         &       -2.28         &        8.29\sym{**} &        8.28\sym{**} &        6.63\sym{*}  &        6.64\sym{*}  \\
                    &      [3.86]         &      [0.16]         &     [-0.06]         &     [-0.24]         &      [2.55]         &      [2.56]         &      [1.94]         &      [1.95]         \\
[1em]
Post                &       -7.61\sym{**} &      -10.96\sym{*}  &       -8.45\sym{**} &       -9.38\sym{***}&       -8.80\sym{***}&       -8.74\sym{***}&       -9.92\sym{***}&       -9.88\sym{***}\\
                    &     [-2.10]         &     [-1.77]         &     [-2.62]         &     [-2.79]         &     [-3.43]         &     [-3.39]         &     [-3.89]         &     [-3.86]         \\
[1em]
\hline
Issuer FE      &                     &$\checkmark$         &$\checkmark$         &$\checkmark$         &$\checkmark$         &$\checkmark$         &$\checkmark$          &$\checkmark$         \\
State-Year FE       &                     &                     &$\checkmark$         &$\checkmark$         &$\checkmark$         &$\checkmark$         &$\checkmark$         &$\checkmark$         \\
Advisor FE             &                     &                     &                     &$\checkmark$         &$\checkmark$         &$\checkmark$         &$\checkmark$         &  $\checkmark$\\
Bond Controls     &                     &                     &                     &                     &$\checkmark$         &$\checkmark$         &$\checkmark$         &$\checkmark$         \\
County Controls           &                     &                     &                     &                     &                     &$\checkmark$         &         &$\checkmark$         \\
Advisor-Year FE          &                     &                     &                     &                     &                     &      & $\checkmark$ &$\checkmark$         \\
Adj.-R$^2$          &       0.052         &       0.337         &       0.454         &       0.461         &       0.856         &       0.857         &       0.863         &       0.863         \\
Obs.                &      56,793         &      51,321         &      51,321         &      51,220         &      51,220         &      51,220         &      50,668         &      50,668         \\
\hline
\end{tabular}
}
\end{table}
\end{landscape}

\begin{landscape}
\begin{table}[htbp]
\def\sym#1{\ifmmode^{#1}\else\(^{#1}\)\fi}
\caption{Impact on Offering Yield Spreads of Local Governments using Issue Yield Spreads} 
\label{table:issu_spread}
\vspace{0.2in}
\par
{\footnotesize This table reports the baseline results for my sample using Equation \eqref{eq:baseline} estimating the differential effect on municipal issue yield spreads of treated and control bonds at the issue level, after the Municipal Advisor Rule of 2014. The primary coefficient of interest, $\beta_0$, is captured by the interaction term of \textit{Treated $\times$ Post}. Specifically, Column (1) reports the results without any controls or fixed effects. In Column (2), I first introduce issuer fixed effects. Column (3) shows results by introducing state $\times$ year fixed effects. In Column (4), I add advisor fixed effect. Column (5) reports the results by additionally including bond level controls consisting of coupon (\%); log(amount issued in \$); dummies for callable bonds, bond insurance, general obligation bond, bank qualification, refunding and credit enhancement; credit rating; remaining years to maturity; and inverse years to maturity. I provide the description of key variables in Table \ref{table:vardescription}. In Column (6), I control for the county-level economic conditions. I use the lagged values for log(labor force) and unemployment rate, and the percentage change in unemployment rate and labor force, respectively. Column (7) replaces advisor fixed effect with advisor $\times$ year fixed effect and does not include county-level controls. Finally, Column (8) shows results by also adding county-level controls. T-statistics are reported in brackets and standard errors are clustered at the state level. \sym{*} \(p<0.10\), \sym{**} \(p<0.05\), \sym{***} \(p<0.01\)}\\
% \vspace{.2in}
\vspace{.05in} 
% \resizebox{0.9\textwidth}{!} {

% \raggedright\textbf{Panel A: Primary Market}\\
\vspace{0.1in}
\centering
\resizebox{1.25\textwidth}{!} {
\begin{tabular}{@{\extracolsep{4pt}}l*{8}{c}}
\hline
                    \emph{Dependent Variable}:&\multicolumn{8}{c}{Issue Level Yield Spread (basis points)}\\
                    \cline{2-9}\\                    &\multicolumn{1}{c}{(1)}&\multicolumn{1}{c}{(2)}&\multicolumn{1}{c}{(3)}&\multicolumn{1}{c}{(4)}&\multicolumn{1}{c}{(5)}&\multicolumn{1}{c}{(6)}&\multicolumn{1}{c}{(7)}&\multicolumn{1}{c}{(8)}\\
                    % &\multicolumn{3}{c}{Yield}&\multicolumn{3}{c}{Spread}&\multicolumn{3}{c}{yield spread}\\
\hline
Treated $\times$ Post &      -34.30\sym{***}&      -33.57\sym{***}&      -14.00\sym{***}&      -12.90\sym{**} &      -14.81\sym{***}&      -14.74\sym{***}&      -14.16\sym{***}&      -14.13\sym{***}\\
                    &     [-4.21]         &     [-4.52]         &     [-2.70]         &     [-2.68]         &     [-4.95]         &     [-4.92]         &     [-4.71]         &     [-4.71]         \\
[1em]
Treated             &       40.00\sym{***}&       -7.23         &        2.35         &        1.03         &        6.74\sym{***}&        6.74\sym{***}&        6.49\sym{**} &        6.51\sym{**} \\
                    &      [4.08]         &     [-0.66]         &      [0.39]         &      [0.17]         &      [3.05]         &      [3.08]         &      [2.49]         &      [2.52]         \\
[1em]
Post                &      -72.93\sym{***}&      -74.34\sym{***}&       -4.50         &       -5.20         &       -5.16\sym{*}  &       -5.05\sym{*}  &       -4.92\sym{*}  &       -4.81\sym{*}  \\
                    &    [-26.09]         &    [-20.66]         &     [-1.46]         &     [-1.59]         &     [-1.87]         &     [-1.83]         &     [-1.78]         &     [-1.74]         \\
[1em]
\hline
Issuer FE      &                     &$\checkmark$         &$\checkmark$         &$\checkmark$         &$\checkmark$         &$\checkmark$         &$\checkmark$          &$\checkmark$         \\
State-Year FE       &                     &                     &$\checkmark$         &$\checkmark$         &$\checkmark$         &$\checkmark$         &$\checkmark$         &$\checkmark$         \\
Advisor FE             &                     &                     &                     &$\checkmark$         &$\checkmark$         &$\checkmark$         &$\checkmark$         &  $\checkmark$\\
Bond Controls     &                     &                     &                     &                     &$\checkmark$         &$\checkmark$         &$\checkmark$         &$\checkmark$         \\
County Controls           &                     &                     &                     &                     &                     &$\checkmark$         &         &$\checkmark$         \\
Advisor-Year FE          &                     &                     &                     &                     &                     &      & $\checkmark$ &$\checkmark$         \\
Adj.-R$^2$          &       0.145         &       0.251         &       0.699         &       0.702         &       0.816         &       0.816         &       0.824         &       0.824         \\
Obs.                &      56,793         &      51,321         &      51,321         &      51,220         &      51,220         &      51,220         &      50,668         &      50,668         \\
\hline
\end{tabular}
}
\end{table}
\end{landscape}

\clearpage
\newpage
\begin{table}[htbp]
% \centering
\def\sym#1{\ifmmode^{#1}\else\(^{#1}\)\fi}
% \scriptsize
\caption{Robustness Tests using Offering Yields}
\label{table:robustness_yld}
\vspace{0.2in}
\par
{\footnotesize In this table I report results for various robustness tests on the baseline specification, i.e., Column (8) of Table \ref{table:main_baseline} with offering yield as the dependent variable. Columns (1)-(2) show the baseline effect by changing the dependent variable to after-tax yield and after-tax yield spread, respectively. In Columns (3)-(11), I report results based on alternative econometric specifications. I introduce additional fixed effects to account for unobserved factors that may be varying over time. Specifically, Column (3) reports baseline results by adding issuer-type $\times$ year fixed effects. Column (4) shows results by adding bond purpose fixed effects. I add bond purpose $\times$ year fixed effect in Column (5). Columns (6) and (7) show results by adding underwriter fixed effect and underwriter $\times$ year fixed effect, respectively. In Columns (8) and (9), I control for unobserved pairing between issuers and advisors, as well as issuers and underwriters, separately, by adding issuer-advisor pair fixed effect and issuer-underwriter pair fixed effect, respectively. These specifications include time unvarying advisor and underwriter fixed effects, respectively. Column (10) shows results with advisor $\times$ state fixed effects. In Column (11), I also add county $\times$ year fixed effects. I consider additional tax considerations in Columns (12)-(14). First, I relax the sample of bonds to include taxable bonds in Columns (12)-(13). In Column (13), I further omit bonds from five states (IL, IA, KS, OK, WI) that tax interest income on municipal bonds issued in-state or out-of-state \citep{gao2021good}. Column (14) shows results using bonds that are exempt from both state and federal income tax simultaneously. Columns (15)-(18) report results focusing on sub-samples of homogeneous bonds. Accordingly, in Column (15), I drop bonds in which the advisor and underwriter are same. Column (16) shows results by dropping callable bonds. I drop insured bonds in Column (17). Finally, I focus on only the new money bonds in Column (18). The results in Columns (19)-(21) focus on additional geographic considerations. I keep only local bonds (by dropping state level bonds) in Column (19). Conversely, I show results using only the state level bonds in Column (20). In Column (21), I report the baseline results by dropping issuances from the three largest municipal bond issuers, namely: California (CA), New York (NY) and Texas (TX). I consider alternative levels of clustering standard errors in Columns (22)-(32). In Columns (22)-(26), I cluster standard errors by advisor, underwriter, issuer, issuer(2), and bond issue, respectively. Issuer(2) in Column (25) refers to weakly identifying borrowers based on the first six-digits of the bond CUSIP \citep{gao2021good}. Columns (27)-(28) double cluster standard errors along two dimensions in the geography of issuers: state-advisor, and advisor-issuer, respectively. Finally, in Columns (29)-(32), I double cluster standard errors over time and across bonds using: state and year, advisor and year, state and year-month, and advisor and year-month, respectively. T-statistics are reported in brackets and standard errors are clustered at the state level, unless otherwise specified. \sym{*} \(p<0.10\), \sym{**} \(p<0.05\), \sym{***} \(p<0.01\)}\\
\end{table}
\clearpage
\newpage
\begin{landscape}
\begin{table}
    \centering
    \def\sym#1{\ifmmode^{#1}\else\(^{#1}\)\fi}
    \vspace{0.2cm}
    \resizebox{1.3\textwidth}{!}{
\begin{tabular}{@{\extracolsep{4pt}}l*{11}{c}@{}}
\hline
                    \emph{Dependent Variable}: &\multicolumn{11}{c}{Offering Yield (basis points)} \vspace{0.2in} \\
                    &\multicolumn{2}{c}{Other Dependent Variables}&\multicolumn{9}{c}{Alternative Specifications}\\
                    \cline{2-3} \cline{4-12}  \\
                    &\multicolumn{1}{c}{After-tax  }&\multicolumn{1}{c}{After-tax }&\multicolumn{1}{c}{Add Issuer-Type}&\multicolumn{1}{c}{Add}&\multicolumn{1}{c}{Add Purpose}&\multicolumn{1}{c}{Add }&\multicolumn{1}{c}{Add }&\multicolumn{1}{c}{Add }&\multicolumn{1}{c}{Add}&\multicolumn{1}{c}{Add}&\multicolumn{1}{c}{Add}\\                   &\multicolumn{1}{c}{Yield}&\multicolumn{1}{c}{Yield Spread}&\multicolumn{1}{c}{Year FE}&\multicolumn{1}{c}{Purpose FE}&\multicolumn{1}{c}{Year FE}&\multicolumn{1}{c}{UW FE}&\multicolumn{1}{c}{UW-Yr. FE}&\multicolumn{1}{c}{Iss.-MA FE}&\multicolumn{1}{c}{Iss.-UW FE}&\multicolumn{1}{c}{MA-State FE}&\multicolumn{1}{c}{County-Yr. FE}\\ &\multicolumn{1}{c}{(1)}&\multicolumn{1}{c}{(2)}&\multicolumn{1}{c}{(3)}&\multicolumn{1}{c}{(4)}&\multicolumn{1}{c}{(5)}&\multicolumn{1}{c}{(6)}&\multicolumn{1}{c}{(7)}&\multicolumn{1}{c}{(8)}&\multicolumn{1}{c}{(9)}&\multicolumn{1}{c}{(10)}&\multicolumn{1}{c}{(11)}\\
\hline\\
\vspace{0.2cm}
Treated $\times$ Post &      -18.13\sym{***}&      -19.69\sym{***}&      -10.51\sym{***}&      -11.08\sym{***}&      -10.61\sym{***}&      -11.00\sym{***}&       -9.29\sym{***}&      -12.61\sym{***}&      -11.43\sym{**} &      -10.25\sym{***}&       -8.57\sym{***}\\
                    &     [-4.23]         &     [-4.33]         &     [-4.02]         &     [-4.06]         &     [-3.89]         &     [-4.18]         &     [-3.14]         &     [-4.28]         &     [-2.44]         &     [-3.81]         &     [-2.87]         \\
[1em]
Adj.-R$^2$          &       0.867         &       0.853         &       0.868         &       0.868         &       0.868         &       0.869         &       0.873         &       0.870         &       0.893         &       0.869         &       0.878         \\
Obs.                &     833,343         &     833,343         &     833,667         &     833,348         &     833,348         &     834,730         &     834,707         &     834,670         &     834,297         &     834,731         &     834,629         \\
\hline
\end{tabular}
}\\

% \vspace{1cm}
\medskip
% \vspace{-2em}
   \resizebox{1.3\textwidth}{!}{
\begin{tabular}{@{\extracolsep{4pt}}l*{10}{c}@{}}

                    \emph{Dependent Variable}: &\multicolumn{10}{c}{Offering Yield (basis points)} \vspace{0.2in}\\
                    \cline{2-11} \\
                    &\multicolumn{3}{c}{Tax Considerations}&\multicolumn{4}{c}{Bond Considerations}&\multicolumn{3}{c}{Geographic Considerations}\\
                    \cline{2-4}  \cline{5-8} \cline{9-11} \\ &\multicolumn{2}{c}{Include Taxable}&\multicolumn{1}{c}{Exempt}&\multicolumn{1}{c}{Drop same}&\multicolumn{1}{c}{Drop}&\multicolumn{1}{c}{Drop}&\multicolumn{1}{c}{Only}&\multicolumn{1}{c}{Keep}&\multicolumn{1}{c}{Keep}&\multicolumn{1}{c}{Drop}\\     \cline{2-3}\vspace{-1em}\\  &\multicolumn{1}{c}{}&\multicolumn{1}{c}{(-Taxable States)}&\multicolumn{1}{c}{(Fed.+State)}&\multicolumn{1}{c}{Adv.-UW. bonds}&\multicolumn{1}{c}{Callable}&\multicolumn{1}{c}{Insured}&\multicolumn{1}{c}{New money}&\multicolumn{1}{c}{Local}&\multicolumn{1}{c}{State}&\multicolumn{1}{c}{CA,NY,TX}\\                    &\multicolumn{1}{c}{(12)}&\multicolumn{1}{c}{(13)}&\multicolumn{1}{c}{(14)}&\multicolumn{1}{c}{(15)}&\multicolumn{1}{c}{(16)}&\multicolumn{1}{c}{(17)}&\multicolumn{1}{c}{(18)}&\multicolumn{1}{c}{(19)}&\multicolumn{1}{c}{(20)}&\multicolumn{1}{c}{(21)}\\
\hline\\
\vspace{0.2cm}
Treated $\times$ Post &      -11.08\sym{***}&       -9.83\sym{***}&      -10.83\sym{***}&      -11.17\sym{***}&      -10.75\sym{***}&      -13.16\sym{***}&      -20.92\sym{***}&       -9.42\sym{***}&      -12.66\sym{**} &      -15.35\sym{***}\\
                    &     [-4.14]         &     [-3.88]         &     [-3.95]         &     [-4.26]         &     [-6.21]         &     [-6.33]         &     [-6.21]         &     [-3.42]         &     [-2.39]         &     [-7.58]         \\
[1em]
Adj.-R$^2$          &       0.868         &       0.865         &       0.866         &       0.867         &       0.828         &       0.870         &       0.879         &       0.875         &       0.838         &       0.871         \\
Obs.                &     834,741         &     737,424         &     770,446         &     830,458         &     443,572         &     698,776         &     415,926         &     751,278         &      83,456         &     519,544         \\
\hline
\end{tabular}
}\\

% \vspace{1cm}
% \vspace{-2em}
\medskip
   \resizebox{1.3\textwidth}{!}{
\begin{tabular}{@{\extracolsep{4pt}}l*{11}{c}@{}}
                    \emph{Dependent Variable}: &\multicolumn{11}{c}{Offering Yield (basis points)} \vspace{0.2in} \\
                    \cline{2-12} \\
                    &\multicolumn{11}{c}{Alternative Clustering}\\
                    \cline{2-12}\\                    &\multicolumn{1}{c}{Advisor}&\multicolumn{1}{c}{Underwriter}&\multicolumn{1}{c}{Issuer}&\multicolumn{1}{c}{Issuer(2)}&\multicolumn{1}{c}{Issue}&\multicolumn{1}{c}{State, Advisor}&\multicolumn{1}{c}{Advisor, Issuer}&\multicolumn{1}{c}{State, Year}&\multicolumn{1}{c}{Advisor, Year}&\multicolumn{1}{c}{State, YM}&\multicolumn{1}{c}{Advisor, YM}\\    &\multicolumn{1}{c}{(22)}&\multicolumn{1}{c}{(23)}&\multicolumn{1}{c}{(24)}&\multicolumn{1}{c}{(25)}&\multicolumn{1}{c}{(26)}&\multicolumn{1}{c}{(27)}&\multicolumn{1}{c}{(28)}&\multicolumn{1}{c}{(29)}&\multicolumn{1}{c}{(30)}&\multicolumn{1}{c}{(31)}&\multicolumn{1}{c}{(32)}\\
\hline\\
\vspace{0.2cm}
Treated $\times$ Post &      -11.08\sym{***}&      -11.08\sym{***}&      -11.08\sym{***}&      -11.08\sym{***}&      -11.08\sym{***}&      -11.08\sym{***}&      -11.08\sym{***}&      -11.08\sym{***}&      -11.08\sym{***}&      -11.08\sym{***}&      -11.08\sym{***}\\
                    &     [-5.11]         &     [-7.25]         &     [-7.24]         &     [-9.91]         &    [-12.47]         &     [-3.92]         &     [-4.75]         &     [-3.96]         &     [-4.09]         &     [-4.13]         &     [-5.02]         \\
[1em]
Adj.-R$^2$          &       0.868         &       0.868         &       0.868         &       0.868         &       0.868         &       0.868         &       0.868         &       0.868         &       0.868         &       0.868         &       0.868         \\
Obs.                &     834,741         &     834,741         &     834,741         &     834,741         &     834,741         &     834,741         &     834,741         &     834,741         &     834,741         &     834,741         &     834,741         \\
\hline
\end{tabular}
}
\end{table}
\end{landscape}

\clearpage
\newpage
\begin{table}[htbp]
% \centering
\def\sym#1{\ifmmode^{#1}\else\(^{#1}\)\fi}
% \scriptsize
\caption{Robustness Tests using Offering Price}
\label{table:robustness_offPrice}
\vspace{0.2in}
\par
{\footnotesize In this table I report results for various robustness tests on the baseline specification, i.e., Column (8) of Table \ref{table:baseline_px} with offering price as the dependent variable. In Columns (1)-(9), I report results based on alternative econometric specifications. I introduce additional fixed effects to account for unobserved factors that may be varying over time. Specifically, Column (1) reports baseline results by adding issuer-type $\times$ year fixed effects. Column (2) shows results by adding bond purpose fixed effects. I add bond purpose $\times$ year fixed effect in Column (3). Columns (4) and (5) show results by adding underwriter fixed effect and underwriter $\times$ year fixed effect, respectively. In Columns (6) and (7), I control for unobserved pairing between issuers and advisors, as well as issuers and underwriters, separately, by adding issuer-advisor pair fixed effect and issuer-underwriter pair fixed effect, respectively. These specifications include time unvarying advisor and underwriter fixed effects, respectively. Column (8) shows results with advisor $\times$ state fixed effects. In Column (9), I also add county $\times$ year fixed effects. I consider additional tax considerations in Columns (10)-(12). First, I relax the sample of bonds to include taxable bonds in Columns (10)-(11). In Column (11), I further omit bonds from five states (IL, IA, KS, OK, WI) that tax interest income on municipal bonds issued in-state or out-of-state \citep{gao2021good}. Column (12) shows results using bonds that are exempt from both state and federal income tax simultaneously. Columns (13)-(16) report results focusing on sub-samples of homogeneous bonds. Accordingly, in Column (13), I drop bonds in which the advisor and underwriter are same. Column (14) shows results by dropping callable bonds. I drop insured bonds in Column (15). Finally, I focus on only the new money bonds in Column (16). The results in Columns (17)-(19) focus on additional geographic considerations. I keep only local bonds (by dropping state level bonds) in Column (17). Conversely, I show results using only the state level bonds in Column (18). In Column (19), I report the baseline results by dropping issuances from the three largest municipal bond issuers, namely: California (CA), New York (NY) and Texas (TX). I consider alternative levels of clustering standard errors in Columns (20)-(30). In Columns (20)-(24), I cluster standard errors by advisor, underwriter, issuer, issuer(2), and bond issue, respectively. Issuer(2) in Column (23) refers to weakly identifying borrowers based on the first six-digits of the bond CUSIP \citep{gao2021good}. Columns (25)-(26) double cluster standard errors along two dimensions in the geography of issuers: state-advisor, and advisor-issuer, respectively. Finally, in Columns (27)-(30), I double cluster standard errors over time and across bonds using: state and year, advisor and year, state and year-month, and advisor and year-month, respectively. T-statistics are reported in brackets and standard errors are clustered at the state level, unless otherwise specified. \sym{*} \(p<0.10\), \sym{**} \(p<0.05\), \sym{***} \(p<0.01\)}\\
\end{table}
\clearpage
\newpage
\begin{landscape}
\begin{table}
    \centering
    \def\sym#1{\ifmmode^{#1}\else\(^{#1}\)\fi}
    \vspace{0.2cm}
    \resizebox{1.3\textwidth}{!}{
\begin{tabular}{@{\extracolsep{4pt}}l*{9}{c}@{}}
\hline
                    \emph{Dependent Variable}: &\multicolumn{9}{c}{Offering Price (per USD 100)} \vspace{0.2in} \\
                    &\multicolumn{9}{c}{Alternative Specifications}\\
                    \cline{2-10}  \\
                    &\multicolumn{1}{c}{Add Issuer-Type}&\multicolumn{1}{c}{Add}&\multicolumn{1}{c}{Add Purpose}&\multicolumn{1}{c}{Add }&\multicolumn{1}{c}{Add }&\multicolumn{1}{c}{Add }&\multicolumn{1}{c}{Add}&\multicolumn{1}{c}{Add}&\multicolumn{1}{c}{Add}\\                   &\multicolumn{1}{c}{Year FE}&\multicolumn{1}{c}{Purpose FE}&\multicolumn{1}{c}{Year FE}&\multicolumn{1}{c}{UW FE}&\multicolumn{1}{c}{UW-Yr. FE}&\multicolumn{1}{c}{Iss.-MA FE}&\multicolumn{1}{c}{Iss.-UW FE}&\multicolumn{1}{c}{MA-State FE}&\multicolumn{1}{c}{County-Yr. FE}\\ &\multicolumn{1}{c}{(1)}&\multicolumn{1}{c}{(2)}&\multicolumn{1}{c}{(3)}&\multicolumn{1}{c}{(4)}&\multicolumn{1}{c}{(5)}&\multicolumn{1}{c}{(6)}&\multicolumn{1}{c}{(7)}&\multicolumn{1}{c}{(8)}&\multicolumn{1}{c}{(9)}\\
\hline\\
\vspace{0.2cm}
Treated $\times$ Post &        1.00\sym{***}&        1.05\sym{***}&        1.02\sym{***}&        1.03\sym{***}&        0.92\sym{***}&        1.11\sym{***}&        0.92\sym{**} &        0.97\sym{***}&        0.84\sym{***}\\
                    &      [4.42]         &      [4.31]         &      [4.33]         &      [4.22]         &      [3.82]         &      [4.44]         &      [2.28]         &      [4.11]         &      [3.51]         \\
[1em]
Adj.-R$^2$          &       0.774         &       0.774         &       0.774         &       0.775         &       0.777         &       0.776         &       0.796         &       0.775         &       0.783         \\
Obs.                &     833,666         &     833,347         &     833,347         &     834,729         &     834,706         &     834,669         &     834,296         &     834,730         &     834,628         \\
\hline
\end{tabular}
}\\

% \vspace{1cm}
\medskip
% \vspace{-2em}
   \resizebox{1.3\textwidth}{!}{
\begin{tabular}{@{\extracolsep{4pt}}l*{10}{c}@{}}

                    \emph{Dependent Variable}: &\multicolumn{10}{c}{Offering Price (per USD 100)} \vspace{0.2in}\\
                    \cline{2-11} \\
                    &\multicolumn{3}{c}{Tax Considerations}&\multicolumn{4}{c}{Bond Considerations}&\multicolumn{3}{c}{Geographic Considerations}\\
                    \cline{2-4}  \cline{5-8} \cline{9-11} \\ &\multicolumn{2}{c}{Include Taxable}&\multicolumn{1}{c}{Exempt}&\multicolumn{1}{c}{Drop same}&\multicolumn{1}{c}{Drop}&\multicolumn{1}{c}{Drop}&\multicolumn{1}{c}{Only}&\multicolumn{1}{c}{Keep}&\multicolumn{1}{c}{Keep}&\multicolumn{1}{c}{Drop}\\     \cline{2-3}\vspace{-1em}\\  &\multicolumn{1}{c}{}&\multicolumn{1}{c}{(-Taxable States)}&\multicolumn{1}{c}{(Fed.+State)}&\multicolumn{1}{c}{Adv.-UW. bonds}&\multicolumn{1}{c}{Callable}&\multicolumn{1}{c}{Insured}&\multicolumn{1}{c}{New money}&\multicolumn{1}{c}{Local}&\multicolumn{1}{c}{State}&\multicolumn{1}{c}{CA,NY,TX}\\                    &\multicolumn{1}{c}{(10)}&\multicolumn{1}{c}{(11)}&\multicolumn{1}{c}{(12)}&\multicolumn{1}{c}{(13)}&\multicolumn{1}{c}{(14)}&\multicolumn{1}{c}{(15)}&\multicolumn{1}{c}{(16)}&\multicolumn{1}{c}{(17)}&\multicolumn{1}{c}{(18)}&\multicolumn{1}{c}{(19)}\\
\hline\\
\vspace{0.2cm}
Treated $\times$ Post &        1.05\sym{***}&        0.94\sym{***}&        1.01\sym{***}&        1.05\sym{***}&        0.72\sym{***}&        1.24\sym{***}&        1.62\sym{***}&        0.90\sym{***}&        1.02\sym{**} &        1.45\sym{***}\\
                    &      [4.36]         &      [3.99]         &      [4.15]         &      [4.43]         &      [4.81]         &      [6.82]         &      [6.99]         &      [3.79]         &      [2.54]         &      [9.28]         \\
[1em]
Adj.-R$^2$          &       0.774         &       0.774         &       0.774         &       0.774         &       0.806         &       0.773         &       0.776         &       0.776         &       0.755         &       0.777         \\
Obs.                &     834,740         &     737,423         &     770,445         &     830,457         &     443,571         &     698,775         &     415,926         &     751,277         &      83,456         &     519,544         \\
\hline
\end{tabular}
}\\

% \vspace{1cm}
% \vspace{-2em}
\medskip
   \resizebox{1.3\textwidth}{!}{
\begin{tabular}{@{\extracolsep{4pt}}l*{11}{c}@{}}
                    \emph{Dependent Variable}: &\multicolumn{11}{c}{Offering Price (per USD 100)} \vspace{0.2in} \\
                    \cline{2-12} \\
                    &\multicolumn{11}{c}{Alternative Clustering}\\
                    \cline{2-12}\\                    &\multicolumn{1}{c}{Advisor}&\multicolumn{1}{c}{Underwriter}&\multicolumn{1}{c}{Issuer}&\multicolumn{1}{c}{Issuer(2)}&\multicolumn{1}{c}{Issue}&\multicolumn{1}{c}{State, Advisor}&\multicolumn{1}{c}{Advisor, Issuer}&\multicolumn{1}{c}{State, Year}&\multicolumn{1}{c}{Advisor, Year}&\multicolumn{1}{c}{State, YM}&\multicolumn{1}{c}{Advisor, YM}\\    &\multicolumn{1}{c}{(20)}&\multicolumn{1}{c}{(21)}&\multicolumn{1}{c}{(22)}&\multicolumn{1}{c}{(23)}&\multicolumn{1}{c}{(24)}&\multicolumn{1}{c}{(25)}&\multicolumn{1}{c}{(26)}&\multicolumn{1}{c}{(27)}&\multicolumn{1}{c}{(28)}&\multicolumn{1}{c}{(29)}&\multicolumn{1}{c}{(30)}\\
\hline\\
\vspace{0.2cm}
Treated $\times$ Post &        1.05\sym{***}&        1.05\sym{***}&        1.05\sym{***}&        1.05\sym{***}&        1.05\sym{***}&        1.05\sym{***}&        1.05\sym{***}&        1.05\sym{***}&        1.05\sym{***}&        1.05\sym{***}&        1.05\sym{***}\\
                    &      [5.14]         &      [7.64]         &      [8.71]         &     [12.49]         &     [15.68]         &      [3.89]         &      [4.89]         &      [3.90]         &      [4.11]         &      [4.26]         &      [4.96]         \\
[1em]
Adj.-R$^2$          &       0.774         &       0.774         &       0.774         &       0.774         &       0.774         &       0.774         &       0.774         &       0.774         &       0.774         &       0.774         &       0.774         \\
Obs.                &     834,740         &     834,740         &     834,740         &     834,740         &     834,740         &     834,740         &     834,740         &     834,740         &     834,740         &     834,740         &     834,740         \\
\hline
\end{tabular}
}
\end{table}
\end{landscape}

\begin{table}[htbp]
\def\sym#1{\ifmmode^{#1}\else\(^{#1}\)\fi}
\caption{Impact Due to Advisor's Ex-ante Role in ``Selecting'' Underwriter} 
\label{table:cs_byUWintro_yld_px}
\vspace{0.2in}
\par
{\footnotesize This table reports the results using Equation \eqref{eq:baseline} to show the differential effect among issuers for whom advisors play a greater role in selecting underwriters. The dependent variable is offering yield spread. I use the average (Columns (1)-(3)) and weighted average (Columns (4)-(6)) of ex-ante likelihood of a new underwriter being introduced by an advisor for a given issuer, respectively. Specifically, I interact the equation with dummies corresponding to below and above median values for this measure among issuers. This analysis also includes group $\times$ year fixed effects. The baseline specification of Column (8) in Table \ref{table:main_baseline} is shown in Columns (3) and (6). T-statistics are reported in brackets and standard errors are clustered at the state level. \sym{*} \(p<0.10\), \sym{**} \(p<0.05\), \sym{***} \(p<0.01\)}\\
% \vspace{.2in}
\vspace{.05in} 
% \resizebox{0.9\textwidth}{!} {

\raggedright\textbf{Panel A: Evidence from Offering Yields}\\
\vspace{0.1in}
\centering
\resizebox{1.0\textwidth}{!} {
\begin{tabular}{@{\extracolsep{4pt}}l*{6}{c}}
\hline
                    \emph{Dependent Variable}:&\multicolumn{6}{c}{Offering Yield (basis points)}\\
                    \cline{2-7}\\ 
                    \emph{Based on Issuers'}:&\multicolumn{3}{c}{Average}&\multicolumn{3}{c}{Weighted Average}\\
                    \cline{2-4}\cline{5-7}\\ 
    Treated $\times$ Post&\multicolumn{1}{c}{(1)}&\multicolumn{1}{c}{(2)}&\multicolumn{1}{c}{(3)}&\multicolumn{1}{c}{(4)}&\multicolumn{1}{c}{(5)}&\multicolumn{1}{c}{(6)}\\
\hline
Below Median       &      -12.60\sym{***}&       -6.82\sym{*}  &       -4.88         &      -12.61\sym{***}&       -6.84\sym{*}  &       -4.90         \\
                    &     [-2.76]         &     [-1.80]         &     [-1.34]         &     [-2.77]         &     [-1.80]         &     [-1.34]         \\
[1em]
Above Median       &      -16.97\sym{***}&      -15.21\sym{***}&      -12.45\sym{***}&      -16.95\sym{***}&      -15.19\sym{***}&      -12.43\sym{***}\\
                    &     [-5.69]         &     [-7.16]         &     [-6.66]         &     [-5.69]         &     [-7.15]         &     [-6.65]         \\
[1em]
\hline
Difference          &        4.37         &        8.39         &        7.57         &        4.34         &        8.36         &        7.52         \\
p-value             &        0.19         &        0.02         &        0.02         &        0.19         &        0.02         &        0.02         \\
Issuer FE           &$\checkmark$         &$\checkmark$         &$\checkmark$         &$\checkmark$         &$\checkmark$         &$\checkmark$         \\
Controls            &$\checkmark$         &$\checkmark$         &$\checkmark$         &$\checkmark$         &$\checkmark$         &$\checkmark$         \\
Advisor FE          &$\checkmark$         &$\checkmark$         &         &$\checkmark$         &$\checkmark$         &         \\
Group-Yr. FE        &$\checkmark$         &$\checkmark$         &$\checkmark$         &$\checkmark$         &$\checkmark$         &$\checkmark$         \\
State-Yr. FE        &                     &$\checkmark$         &$\checkmark$         &                     &$\checkmark$         &$\checkmark$         \\
Advisor-Yr. FE      &                     &                     &$\checkmark$         &                     &                     &$\checkmark$         \\
Adj.-R$^2$          &       0.858         &       0.863         &       0.868         &       0.858         &       0.863         &       0.868         \\
Obs.                &     776,304         &     776,304         &     776,286         &     776,304         &     776,304         &     776,286         \\
\hline
\end{tabular}
}
\end{table}

\begin{table}
\def\sym#1{\ifmmode^{#1}\else\(^{#1}\)\fi}
\raggedright\textbf{Panel B: Evidence from Offering Price}\\
\vspace{0.1in}
\centering
\resizebox{0.9\textwidth}{!} {
\begin{tabular}{@{\extracolsep{4pt}}l*{6}{c}}
\hline
                    \emph{Dependent Variable}:&\multicolumn{6}{c}{Offering Price (per USD 100)}\\
                    \cline{2-7}\\ 
 \emph{Issuers' reliance}:&\multicolumn{3}{c}{Average }&\multicolumn{3}{c}{Wtd. average}\\
                    \cline{2-4}\cline{5-7}\\ 
    Treated $\times$ Post&\multicolumn{1}{c}{(1)}&\multicolumn{1}{c}{(2)}&\multicolumn{1}{c}{(3)}&\multicolumn{1}{c}{(4)}&\multicolumn{1}{c}{(5)}&\multicolumn{1}{c}{(6)}\\
\hline
Below Median       &        0.98\sym{**} &        0.52         &        0.40         &        0.98\sym{**} &        0.52         &        0.40         \\
                    &      [2.43]         &      [1.50]         &      [1.26]         &      [2.43]         &      [1.50]         &      [1.26]         \\
[1em]
Above Median       &        1.47\sym{***}&        1.36\sym{***}&        1.20\sym{***}&        1.47\sym{***}&        1.36\sym{***}&        1.20\sym{***}\\
                    &      [5.66]         &      [7.27]         &      [6.76]         &      [5.66]         &      [7.27]         &      [6.77]         \\
[1em]
\hline
Difference          &       -0.50         &       -0.84         &       -0.81         &       -0.49         &       -0.84         &       -0.80         \\
p-value             &        0.06         &        0.00         &        0.00         &        0.06         &        0.00         &        0.00         \\
Issuer FE           &$\checkmark$         &$\checkmark$         &$\checkmark$         &$\checkmark$         &$\checkmark$         &$\checkmark$         \\
Controls            &$\checkmark$         &$\checkmark$         &$\checkmark$         &$\checkmark$         &$\checkmark$         &$\checkmark$         \\
Advisor FE          &$\checkmark$         &$\checkmark$         &         &$\checkmark$         &$\checkmark$         &         \\
Group-Yr. FE        &$\checkmark$         &$\checkmark$         &$\checkmark$         &$\checkmark$         &$\checkmark$         &$\checkmark$         \\
State-Yr. FE        &                     &$\checkmark$         &$\checkmark$         &                     &$\checkmark$         &$\checkmark$         \\
Advisor-Yr. FE      &                     &                     &$\checkmark$         &                     &                     &$\checkmark$         \\
Adj.-R$^2$          &       0.762         &       0.766         &       0.772         &       0.762         &       0.766         &       0.772         \\
Obs.                &     776,303         &     776,303         &     776,285         &     776,303         &     776,303         &     776,285         \\
\hline
\end{tabular}
}
\end{table}

\begin{table}[htbp]
\def\sym#1{\ifmmode^{#1}\else\(^{#1}\)\fi}
\caption{Heterogeneity by Size of Issuers} 
\label{table:cs_bySize_yld}
\vspace{0.2in}
\par
{\footnotesize This table reports the results using Equation \eqref{eq:baseline} to show the differential effect among issuers based on their ex-ante size. The dependent variable is offering yields. I use the average (Columns (1)-(3)) and median (Columns (4)-(6)) size of ex-ante issuances, respectively. Specifically, I interact the equation with dummies corresponding to small and large values for this measure among issuers. This analysis also includes group $\times$ year fixed effects. The baseline specification of Column (8) in Table \ref{table:main_baseline} is shown in Columns (3) and (6). T-statistics are reported in brackets and standard errors are clustered at the state level. \sym{*} \(p<0.10\), \sym{**} \(p<0.05\), \sym{***} \(p<0.01\)}\\
% \vspace{.2in}
\vspace{.05in} 
% \resizebox{0.9\textwidth}{!} {

% \raggedright\textbf{Panel A: Evidence from Offering Yields}\\
\vspace{0.1in}
\centering
\resizebox{1.0\textwidth}{!} {
\begin{tabular}{@{\extracolsep{4pt}}l*{6}{c}}
\hline
                    \emph{Dependent Variable}:&\multicolumn{6}{c}{Offering Yields (basis points)}\\
                    \cline{2-7}\\ 
                    \emph{Based on Issuers'}:&\multicolumn{3}{c}{Average Size}&\multicolumn{3}{c}{Median Size}\\
                    \cline{2-4}\cline{5-7}\\ 
    Treated $\times$ Post&\multicolumn{1}{c}{(1)}&\multicolumn{1}{c}{(2)}&\multicolumn{1}{c}{(3)}&\multicolumn{1}{c}{(4)}&\multicolumn{1}{c}{(5)}&\multicolumn{1}{c}{(6)}\\
\hline
$\times$ Small&       -9.29         &       -3.34         &       -2.49         &       -8.14         &       -2.84         &       -2.05         \\
                    &     [-1.41]         &     [-0.55]         &     [-0.40]         &     [-1.26]         &     [-0.47]         &     [-0.34]         \\
[1em]
$\times$ Large&      -17.84\sym{***}&      -15.17\sym{***}&      -12.19\sym{***}&      -18.23\sym{***}&      -15.72\sym{***}&      -12.68\sym{***}\\
                    &     [-6.32]         &     [-7.68]         &     [-6.67]         &     [-6.80]         &     [-8.33]         &     [-7.42]         \\
[1em]
\hline
Difference          &        8.55         &       11.83         &        9.70         &       10.09         &       12.88         &       10.63         \\
p-value             &        0.11         &        0.02         &        0.08         &        0.07         &        0.02         &        0.07         \\
Issuer FE           &$\checkmark$         &$\checkmark$         &$\checkmark$         &$\checkmark$         &$\checkmark$         &$\checkmark$         \\
Controls            &$\checkmark$         &$\checkmark$         &$\checkmark$         &$\checkmark$         &$\checkmark$         &$\checkmark$         \\
Advisor FE          &$\checkmark$         &$\checkmark$         &$\checkmark$         &$\checkmark$         &$\checkmark$         &$\checkmark$         \\
Group-Yr. FE        &$\checkmark$         &$\checkmark$         &$\checkmark$         &$\checkmark$         &$\checkmark$         &$\checkmark$         \\
State-Yr. FE        &                     &$\checkmark$         &$\checkmark$         &                     &$\checkmark$         &$\checkmark$         \\
Advisor-Yr. FE      &                     &                     &$\checkmark$         &                     &                     &$\checkmark$         \\
Adj.-R$^2$          &       0.858         &       0.863         &       0.868         &       0.858         &       0.863         &       0.868         \\
Obs.                &     834,760         &     834,760         &     834,741         &     834,760         &     834,760         &     834,741         \\
\hline
\end{tabular}
}
\end{table}

\begin{table}[htbp]
\def\sym#1{\ifmmode^{#1}\else\(^{#1}\)\fi}
\caption{Evidence from the Exit of Municipal Advisors (MA) - lower dependence} 
\label{table:exitingMA_over25}
\vspace{0.2in}
\par
{\footnotesize This table reports the results using Equation \eqref{eq:baseline} with interactions to show the differential effect among issuers based on the exit of municipal advisors (MA). This analysis also includes group $\times$ year fixed effects. Column (1) shows results among all issuers with interactions corresponding to whether the issuer primarily depended on an exiting  advisor or not. I define issuers linked to advisors when more than 25\% of their municipal debt issuance in the pre-period is advised by the exiting advisor. I focus on the exit of regular advisors. These represent municipal advisors with at lease one issuance in each calendar year before the SEC Municipal Advisor Rule in the sample. Columns (2) and (3) show results for issuers that depend on exiting advisors. For these issuers, I show the heterogeneity between small and large issuers based on the median size of ex-ante issuances. Column (2) shows results for advised bonds only. Column (3) also includes bonds issued without any advisors, and the analysis does not include advisor $\times$ year fixed effects. T-statistics are reported in brackets and standard errors are clustered at the state level. \sym{*} \(p<0.10\), \sym{**} \(p<0.05\), \sym{***} \(p<0.01\)}\\
% \vspace{.2in}
\vspace{.05in} 
% \resizebox{0.9\textwidth}{!} {

% \raggedright\textbf{Panel A: Primary Market}\\
\vspace{0.1in}
\centering
\resizebox{0.7\textwidth}{!} {
\begin{tabular}{@{\extracolsep{4pt}}l*{3}{c}}
\hline
                    \emph{Dependent Variable}:&\multicolumn{3}{c}{Yield Spread (basis points)}\\
                    \cline{2-4} \\
                    \emph{Sample of Issuers}:&\multicolumn{1}{c}{All}&\multicolumn{2}{c}{Depending on Exiting MA}\\
                    \cline{2-2} \cline{3-4} \\
Treated $\times$ Post&\multicolumn{1}{c}{(1)}&\multicolumn{1}{c}{(2)}&\multicolumn{1}{c}{(3)}\\
\hline
$\times$ Other   &      -16.93\sym{***}&                     &                     \\
                    &     [-5.58]         &                     &                     \\
[1em]
$\times$ Depend on Exiting MA     &       -1.80         &                     &                     \\
                    &     [-0.49]         &                     &                     \\
[1em]
$\times$ Small      &                     &       14.69\sym{***}&       12.46         \\
                    &                     &      [3.74]         &      [1.56]         \\
[1em]
$\times$ Large      &                     &       -8.85\sym{***}&       -8.53\sym{***}\\
                    &                     &     [-2.70]         &     [-2.85]         \\
[1em]
\hline
Difference          &       -15.13         &       23.54         &       20.98         \\
p-value             &        0.00         &        0.00         &        0.02         \\
Issuer FE           &$\checkmark$         &$\checkmark$         &$\checkmark$         \\
State-Yr. FE        &$\checkmark$         &$\checkmark$         &$\checkmark$         \\
Controls       &$\checkmark$  &$\checkmark$         &$\checkmark$         \\
Group-Yr. FE          &$\checkmark$         &$\checkmark$         &$\checkmark$         \\
Advisor-Yr. FE          &$\checkmark$         &$\checkmark$         &         \\
Adj.-R$^2$          &       0.855         &       0.860         &       0.850         \\
Obs.                &     834,741         &     250,538         &     294,592         \\
\hline
\end{tabular}
}
\end{table}

\begin{table}[htbp]
\def\sym#1{\ifmmode^{#1}\else\(^{#1}\)\fi}
\caption{Evidence from the Exit of Municipal Advisors (MA) - by size of average issuance} 
\label{table:exitingMA_over50_mu}
\vspace{0.2in}
\par
{\footnotesize This table reports the results using Equation \eqref{eq:baseline} with interactions to show the differential effect among issuers based on the exit of municipal advisors (MA). This analysis also includes group $\times$ year fixed effects. Column (1) shows results among all issuers with interactions corresponding to whether the issuer primarily depended on an exiting  advisor or not. I define issuers linked to advisors when more than 25\% of their municipal debt issuance in the pre-period is advised by the exiting advisor. I focus on the exit of regular advisors. These represent municipal advisors with at lease one issuance in each calendar year before the SEC Municipal Advisor Rule in the sample. Columns (2) and (3) show results for issuers that depend on exiting advisors. For these issuers, I show the heterogeneity between small and large issuers based on the average size of ex-ante issuances. Column (2) shows results for advised bonds only. Column (3) also includes bonds issued without any advisors, and the analysis does not include advisor $\times$ year fixed effects. T-statistics are reported in brackets and standard errors are clustered at the state level. \sym{*} \(p<0.10\), \sym{**} \(p<0.05\), \sym{***} \(p<0.01\)}\\
% \vspace{.2in}
\vspace{.05in} 
% \resizebox{0.9\textwidth}{!} {

% \raggedright\textbf{Panel A: Primary Market}\\
\vspace{0.1in}
\centering
\resizebox{0.7\textwidth}{!} {
\begin{tabular}{@{\extracolsep{4pt}}l*{3}{c}}
\hline
                    \emph{Dependent Variable}:&\multicolumn{3}{c}{Yield Spread (basis points)}\\
                    \cline{2-4} \\
                    \emph{Sample of Issuers}:&\multicolumn{1}{c}{All}&\multicolumn{2}{c}{Depending on Exiting MA}\\
                    \cline{2-2} \cline{3-4} \\
Treated $\times$ Post&\multicolumn{1}{c}{(1)}&\multicolumn{1}{c}{(2)}&\multicolumn{1}{c}{(3)}\\
\hline
$\times$ Other   &      -16.61\sym{***}&                     &                     \\
                    &     [-5.60]         &                     &                     \\
[1em]
$\times$ Depend on Exiting MA     &       -0.73         &                     &                     \\
                    &     [-0.22]         &                     &                     \\
[1em]
$\times$ Small      &                     &       15.30\sym{***}&       14.96\sym{**} \\
                    &                     &      [5.66]         &      [2.52]         \\
[1em]
$\times$ Large      &                     &       -5.62         &       -6.17\sym{*}  \\
                    &                     &     [-1.49]         &     [-1.94]         \\
[1em]
\hline
Difference          &       -15.87         &       20.92         &       21.13         \\
p-value             &        0.00         &        0.00         &        0.00         \\
Issuer FE           &$\checkmark$         &$\checkmark$         &$\checkmark$         \\
State-Yr. FE        &$\checkmark$         &$\checkmark$         &$\checkmark$         \\
Controls       &$\checkmark$  &$\checkmark$         &$\checkmark$         \\
Group-Yr. FE          &$\checkmark$         &$\checkmark$         &$\checkmark$         \\
Advisor-Yr. FE          &$\checkmark$         &$\checkmark$         &         \\
Adj.-R$^2$          &       0.855         &       0.861         &       0.854         \\
Obs.                &     834,741         &     234,679         &     275,381         \\
\hline
\end{tabular}
}
\end{table}

\begin{table}[htbp]
\def\sym#1{\ifmmode^{#1}\else\(^{#1}\)\fi}
\caption{Evidence from Refunding Bonds} 
\label{table:refunding}
\vspace{0.2in}
\par
{\footnotesize This table reports the baseline results for the sample of refunding bonds using Equation \eqref{eq:baseline} estimating the differential effect on yield spreads of treated and control bonds after the Municipal Advisor Rule of 2014. The primary coefficient of interest, $\beta_0$, is captured by the interaction term of \textit{Treated $\times$ Post}. I include the full set of controls and fixed effects in each Column corresponding to the baseline specification in Column (8) of Table \ref{table:main_baseline}, showing results for different dependent variables. Specifically, Column (1) reports the results using offering yields as the outcome. I use the after-tax yields as the dependent variable in Column (2). For Column (3), I use the preferred dependent variable in the form of yield spread. Finally, Column (4) shows the effect on after-tax yield spreads. I provide the description of key variables in Table \ref{table:vardescription}. T-statistics are reported in brackets and standard errors are clustered at the state level. \sym{*} \(p<0.10\), \sym{**} \(p<0.05\), \sym{***} \(p<0.01\)}\\
% \vspace{.2in}
\vspace{.05in} 
% \resizebox{0.9\textwidth}{!} {

% \raggedright\textbf{Panel A: Primary Market}\\
\vspace{0.1in}
\centering
\resizebox{1.0\textwidth}{!} {
\begin{tabular}{@{\extracolsep{4pt}}l*{4}{c}}
\hline
                    \emph{Dependent Variable}:&\multicolumn{1}{c}{Offering }&\multicolumn{1}{c}{After-tax }&\multicolumn{1}{c}{Yield }&\multicolumn{1}{c}{After-tax}\\
                    &\multicolumn{1}{c}{Yield (bps)}&\multicolumn{1}{c}{Yield (bps)}&\multicolumn{1}{c}{Spread (bps)}&\multicolumn{1}{c}{Yield Spread (bps)}\\
                &\multicolumn{1}{c}{(1)}&\multicolumn{1}{c}{(2)}&\multicolumn{1}{c}{(3)}&\multicolumn{1}{c}{(4)}\\
\hline
Treated $\times$ Post &       -7.93\sym{***}&      -11.93\sym{***}&       -7.54\sym{***}&      -11.75\sym{***}\\
                    &     [-2.95]         &     [-2.82]         &     [-3.07]         &     [-2.97]         \\
[1em]
Treated             &        7.10\sym{**} &       11.13\sym{**} &        6.39\sym{***}&       10.37\sym{***}\\
                    &      [2.59]         &      [2.52]         &      [2.77]         &      [2.69]         \\
[1em]
Post                &       -8.19\sym{***}&      -14.90\sym{***}&       -6.14\sym{***}&      -12.78\sym{***}\\
                    &     [-5.62]         &     [-5.76]         &     [-2.92]         &     [-4.09]         \\
[1em]
\hline
Issuer FE      &$\checkmark$         &$\checkmark$         &$\checkmark$         &$\checkmark$         \\
Bond Controls       &$\checkmark$         &$\checkmark$         &$\checkmark$         &$\checkmark$         \\
County Controls     &$\checkmark$         &$\checkmark$         &$\checkmark$         &$\checkmark$         \\
State-Yr. FE        &$\checkmark$         &$\checkmark$         &$\checkmark$         &$\checkmark$         \\
Advisor-Yr. FE          &$\checkmark$         &$\checkmark$         &$\checkmark$         &$\checkmark$         \\
Adj.-R$^2$          &       0.880         &       0.880         &       0.864         &       0.865         \\
Obs.                &     418,989         &     418,318         &     418,623         &     417,952         \\
\hline
\end{tabular}
}
\end{table}

\begin{table}[htbp]
\def\sym#1{\ifmmode^{#1}\else\(^{#1}\)\fi}
\caption{Evidence from Timing of pre-refundings}
%See table: Table10__calling_typeL_CCtrl_diff_refIssue_w1
\label{table:timing_refunding_typeL}
\vspace{0.2in}
\par
{\footnotesize This table reports the baseline results for the sample using Equation \eqref{eq:baseline} estimating the differential effect on the timing of pre-refunding bonds for the treated and control bonds after the Municipal Advisor Rule of 2014. I restrict the sample to bonds that are pre-refunded and are callable. In Columns (1)-(6), I focus on all bonds with call option unlocking during the sample period. The primary coefficient of interest, $\beta_0$, is captured by the interaction term of \textit{Treated $\times$ Post}. Our dependent variable is the gap between calling and refunding dates (in days) for bonds in Columns (1)-(5). I use the logged transformation of gap days in Columns (6) as the dependent variable. Specifically, Column (1) reports the results with issuer fixed effects. Column (2) shows results by additionally including state $\times$ year fixed effects. In Column (3), I include advisor fixed effects. Column (4) shows results with bond level controls consisting of coupon (\%); log(amount issued in \$); dummies for callable bonds, bond insurance, general obligation bond, bank qualification, refunding, and credit enhancement; remaining years to maturity; and inverse years to maturity. I provide the description of key variables in Table \ref{table:vardescription}. In Column (5), I control for the county-level economic conditions. I use the lagged values for log(labor force) and unemployment rate, and the percentage change in unemployment rate and labor force, respectively. Column (6) shows the results with logged value of gap days as the dependent variable. T-statistics are reported in brackets and standard errors are clustered at the state level. \sym{*} \(p<0.10\), \sym{**} \(p<0.05\), \sym{***} \(p<0.01\)}\\
% \vspace{.2in}
\vspace{.05in} 
% \resizebox{0.9\textwidth}{!} {

% \raggedright\textbf{Panel A: Primary Market}\\
\vspace{0.1in}
\centering
\resizebox{1.0\textwidth}{!} {
\begin{tabular}{@{\extracolsep{4pt}}l*{6}{c}}
\hline
                    \emph{Dependent Variable}:&\multicolumn{5}{c}{$\Delta$(Calling - Refunding) in days}&\multicolumn{1}{c}{Log($\Delta$)}\\
                    \cline{2-6}\\ &\multicolumn{1}{c}{(1)}&\multicolumn{1}{c}{(2)}&\multicolumn{1}{c}{(3)}&\multicolumn{1}{c}{(4)}&\multicolumn{1}{c}{(5)}&\multicolumn{1}{c}{(6)}\\
\hline
Treated $\times$ Post &     -147.39\sym{**} &     -144.21\sym{**} &     -139.16\sym{**} &     -143.48\sym{**} &     -143.39\sym{**} &       -0.23\sym{*}  \\
                    &     [-2.07]         &     [-2.26]         &     [-2.14]         &     [-2.13]         &     [-2.17]         &     [-1.70]         \\
[1em]
Treated             &       42.60         &       51.16         &       44.44         &       21.20         &       16.83         &       -0.14\sym{*}  \\
                    &      [0.78]         &      [0.99]         &      [0.88]         &      [0.47]         &      [0.38]         &     [-1.72]         \\
[1em]
Post                &       -6.63         &       68.57         &       71.66\sym{*}  &       78.22\sym{*}  &       77.27\sym{*}  &        0.02         \\
                    &     [-0.30]         &      [1.61]         &      [1.75]         &      [1.77]         &      [1.71]         &      [0.21]         \\
[1em]
\hline
Issuer FE           &$\checkmark$         &$\checkmark$         &$\checkmark$         &$\checkmark$         &$\checkmark$         &$\checkmark$         \\
State-Yr. FE        &                     &$\checkmark$         &$\checkmark$         &$\checkmark$         &$\checkmark$         &$\checkmark$         \\
Advisor FE          &                     &                     &$\checkmark$         &$\checkmark$         &$\checkmark$         &$\checkmark$         \\
Bond Controls       &                     &                     &                     &$\checkmark$         &$\checkmark$         &$\checkmark$         \\
County Controls     &                     &                     &                     &                     &$\checkmark$         &$\checkmark$         \\
Adj.-R$^2$          &       0.491         &       0.561         &       0.583         &       0.611         &       0.612         &       0.654         \\
Obs.                &     131,841         &     131,840         &     131,838         &     131,838         &     131,838         &     130,572         \\
\hline
\end{tabular}
}
\end{table}
